# Supplementary material for: GeoDiffuser: Geometry-Based Image Editing with Diffusion Models
Source: arXiv:2404.14403 source file (2025-01-02)

# 2D & 3D Edits

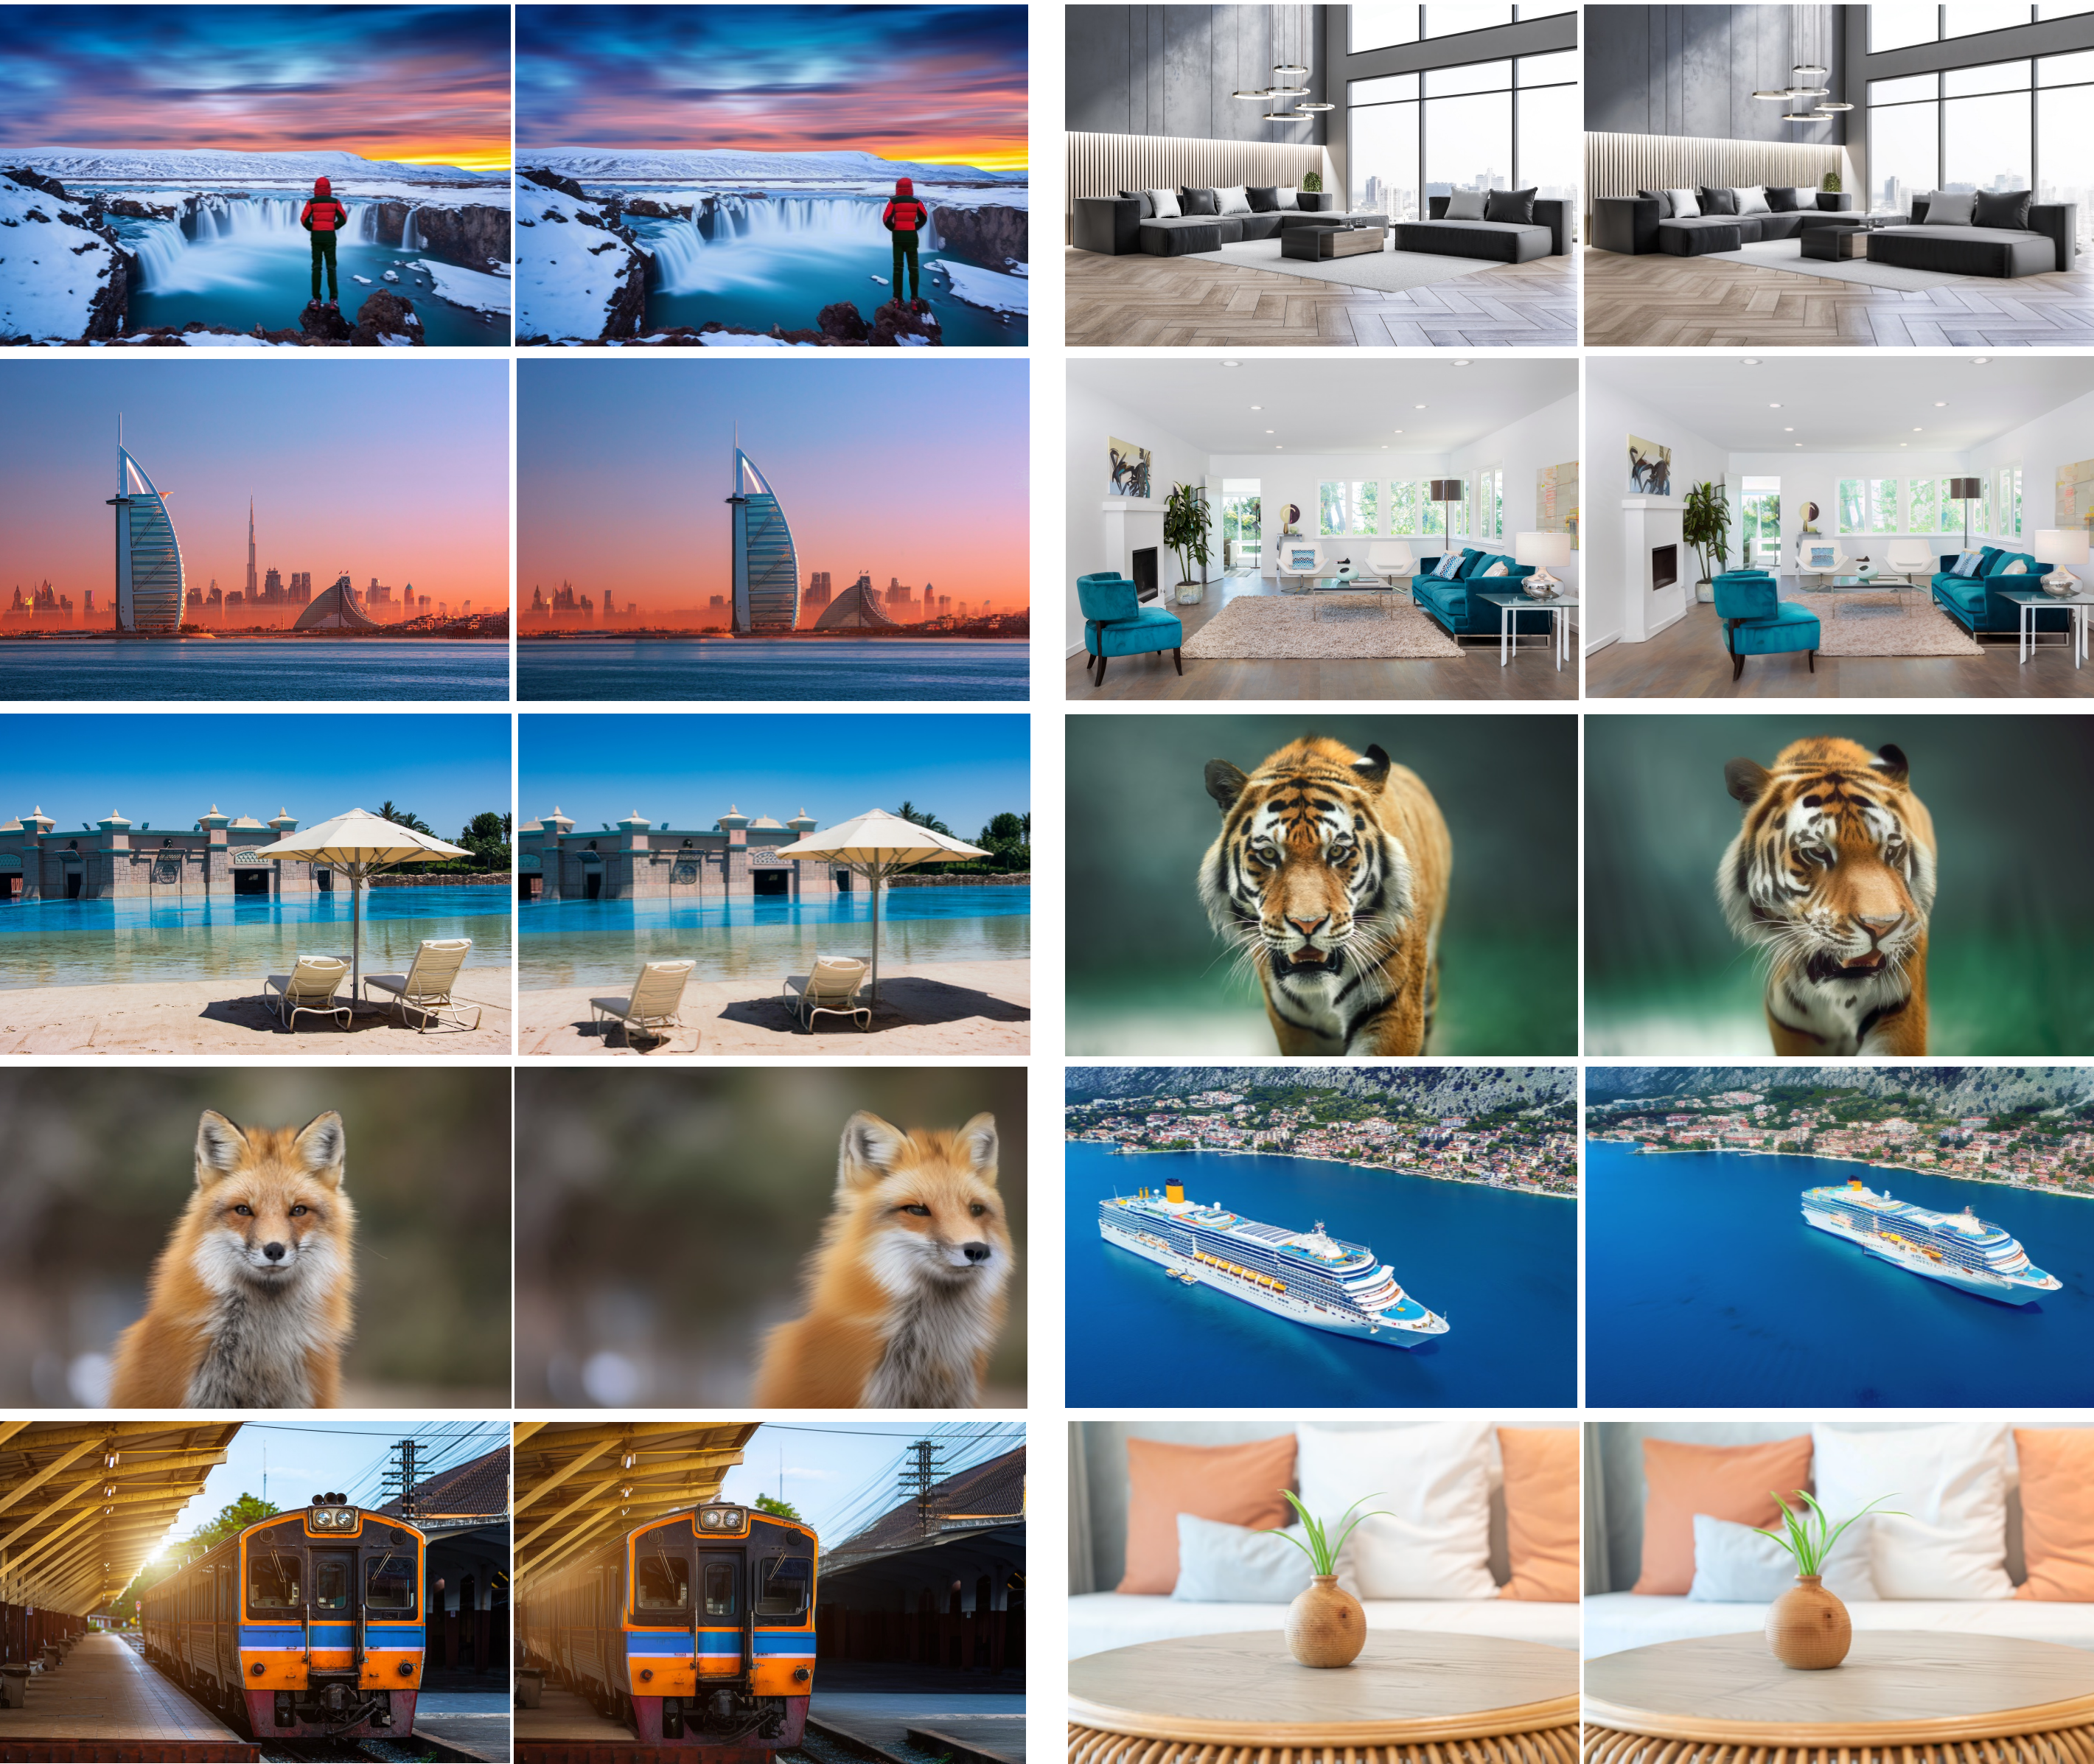

# Removal

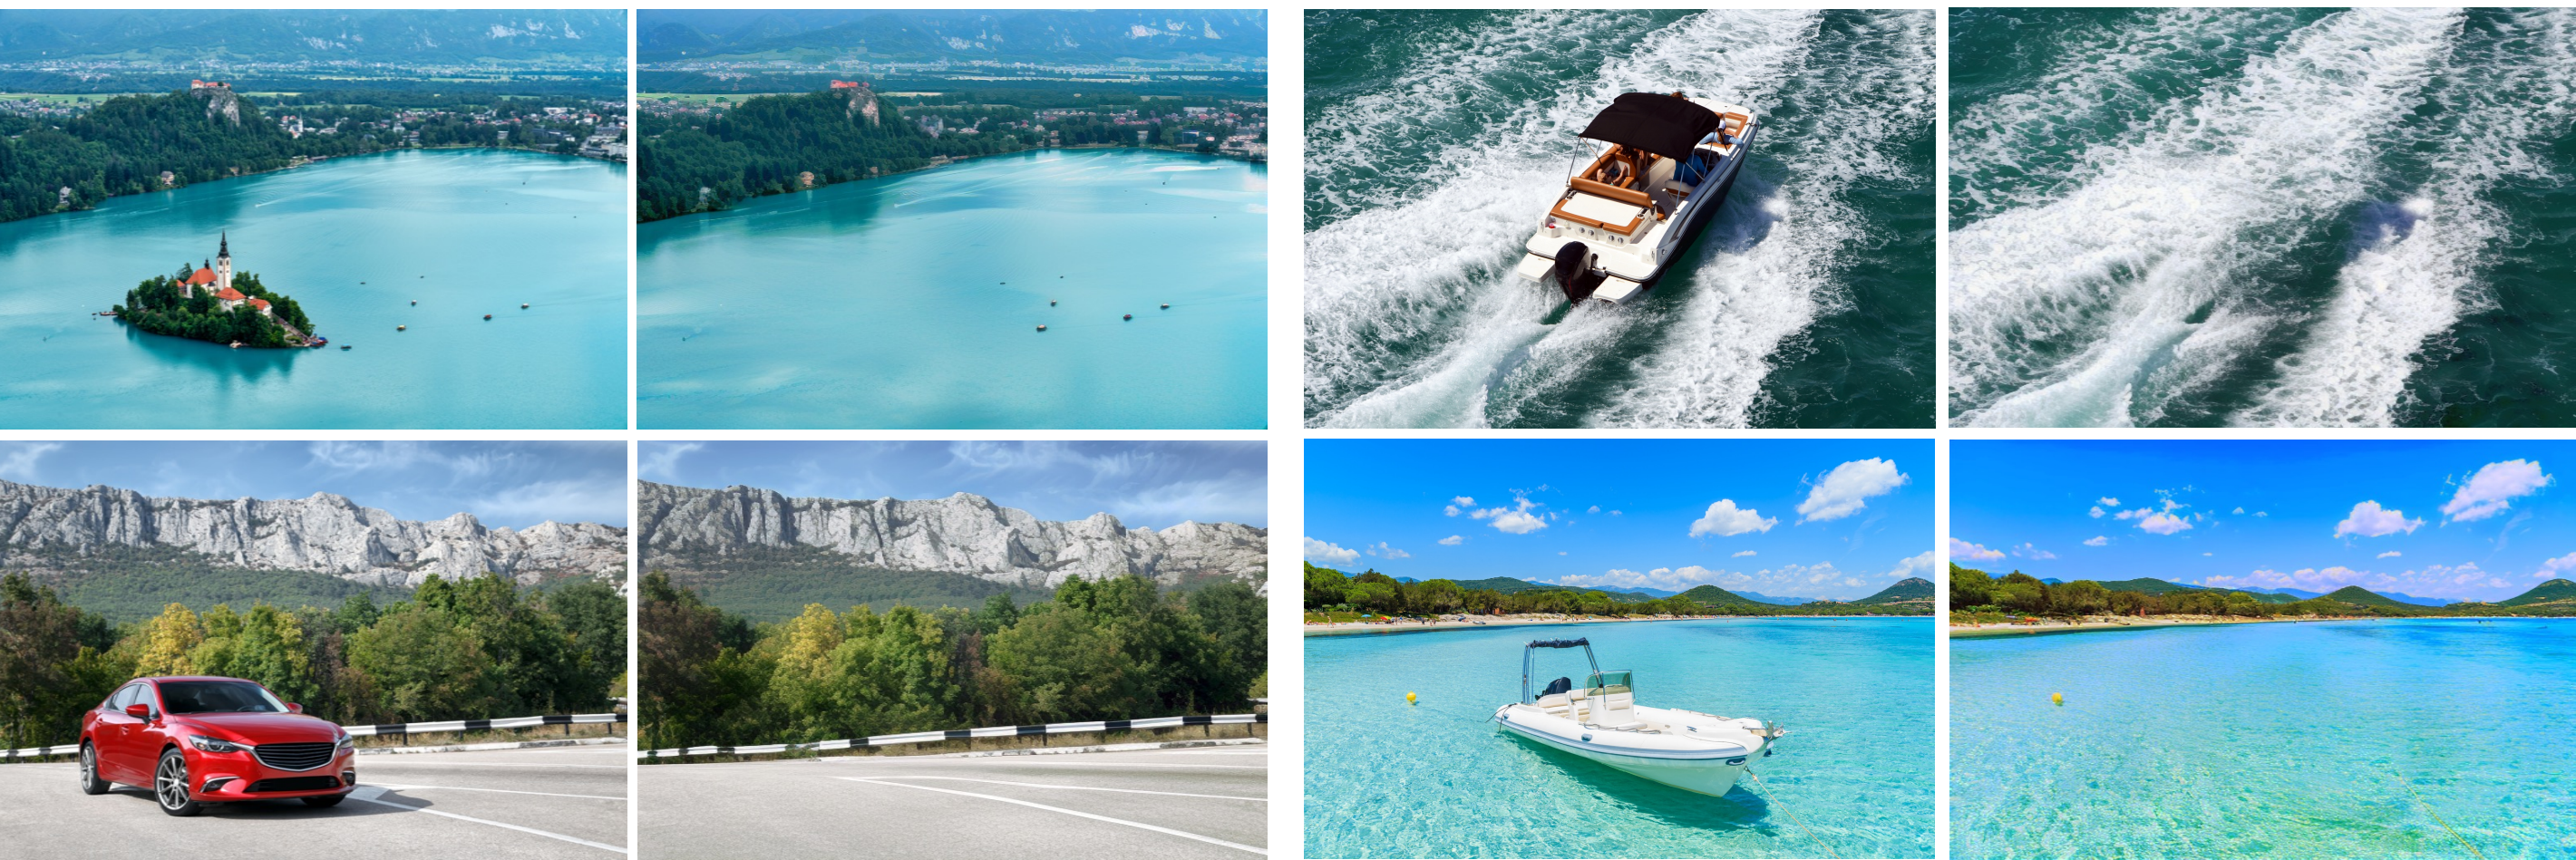



# 2D & 3D Edits

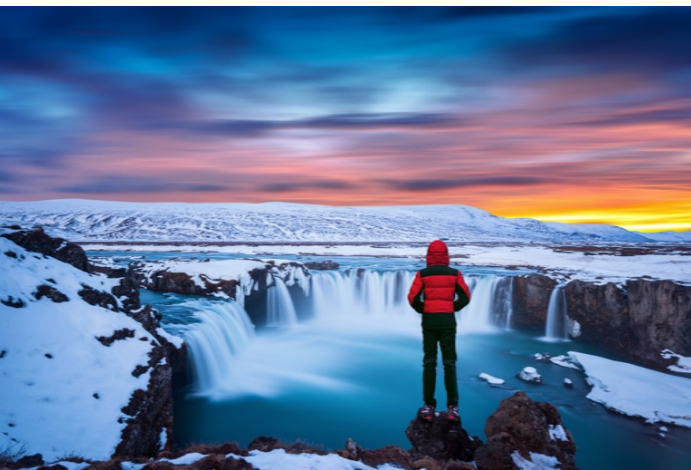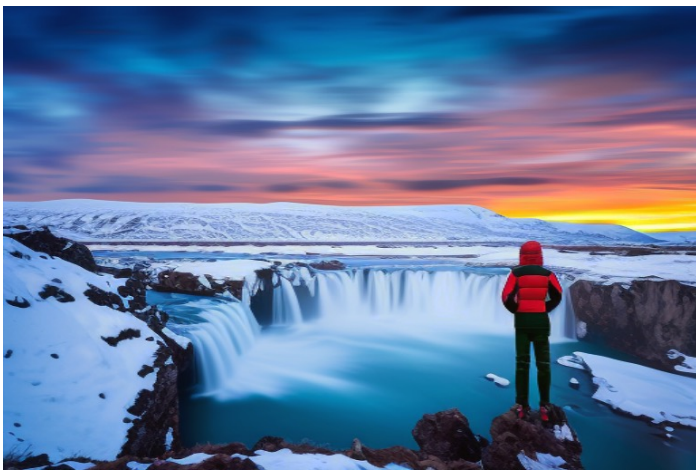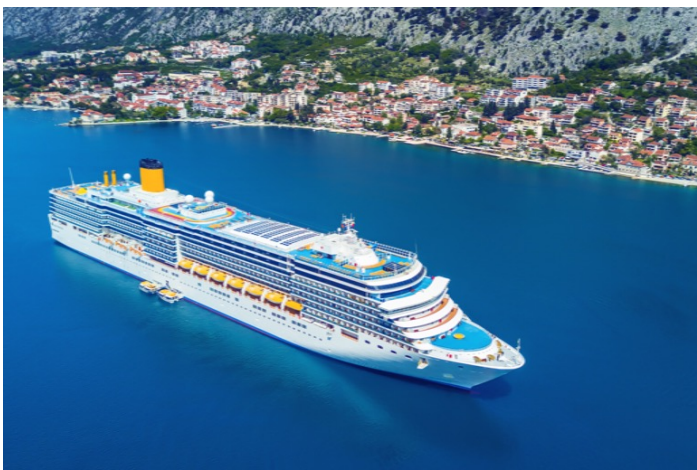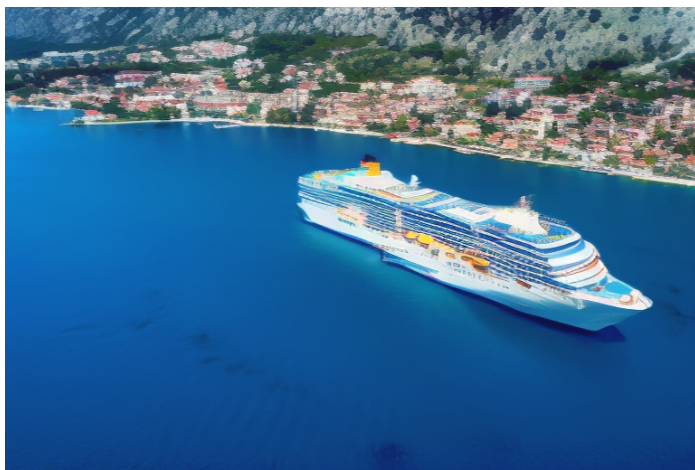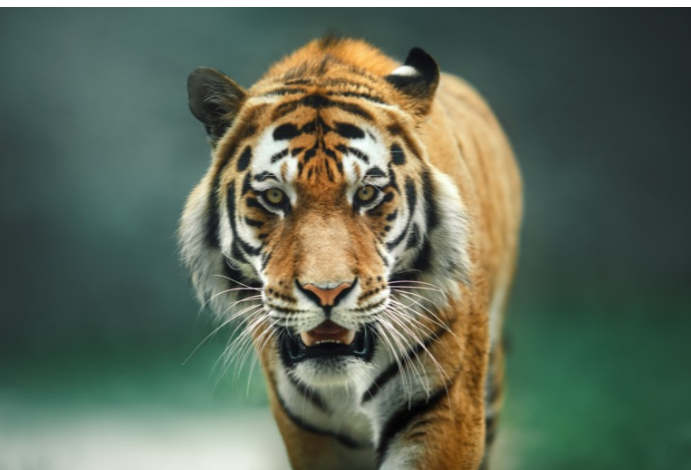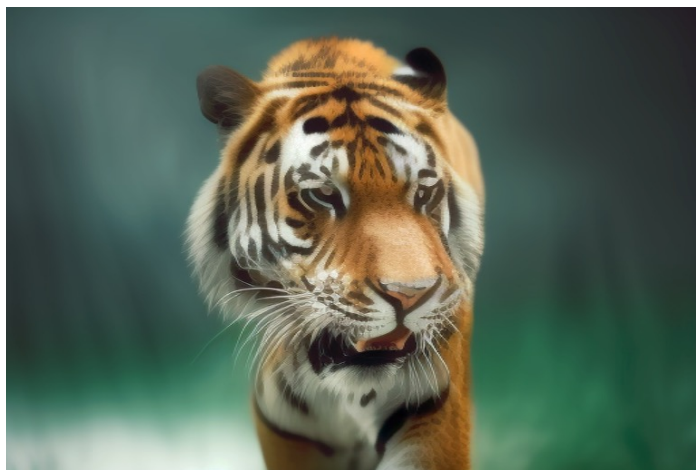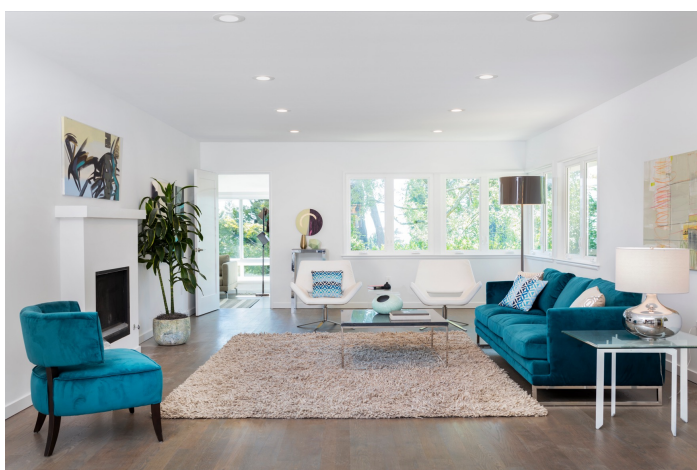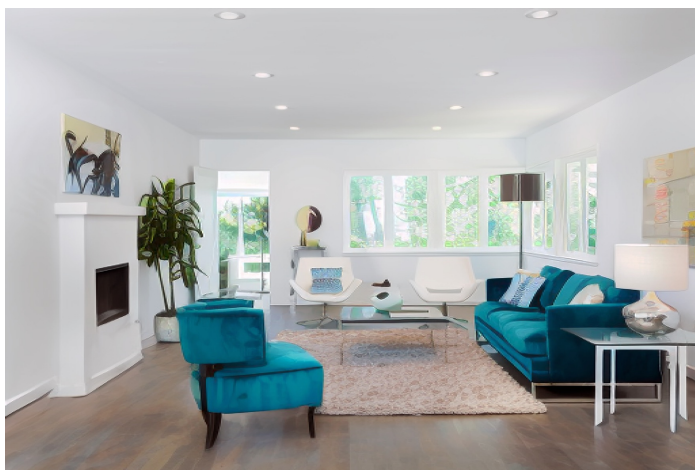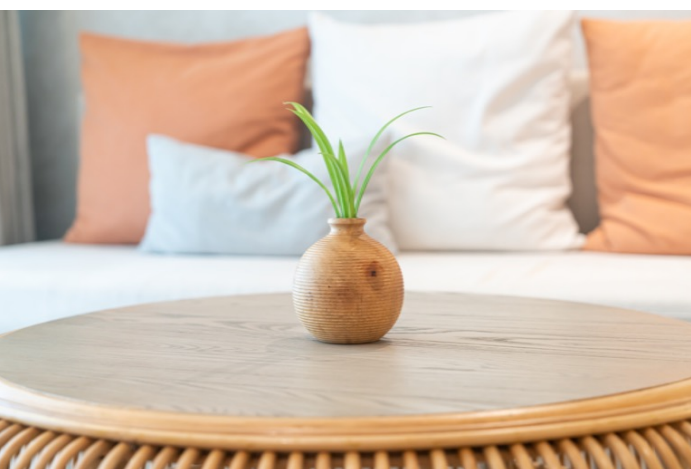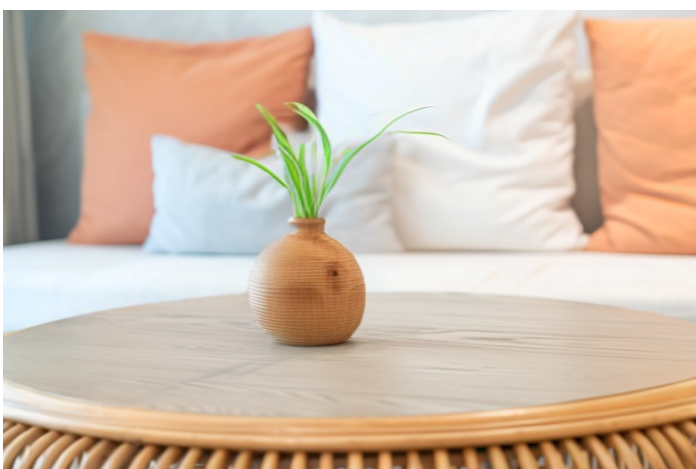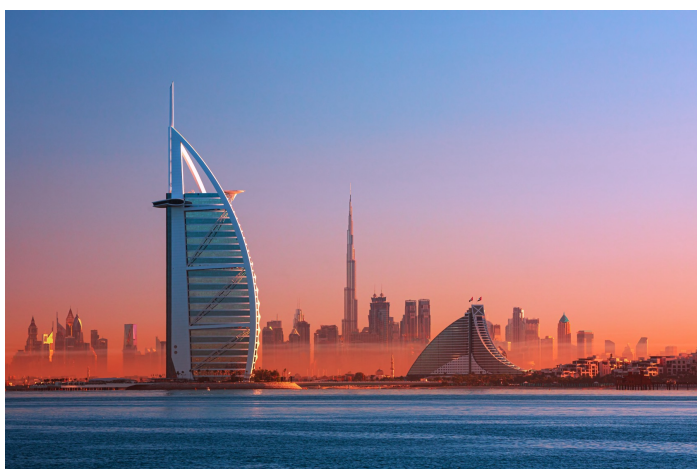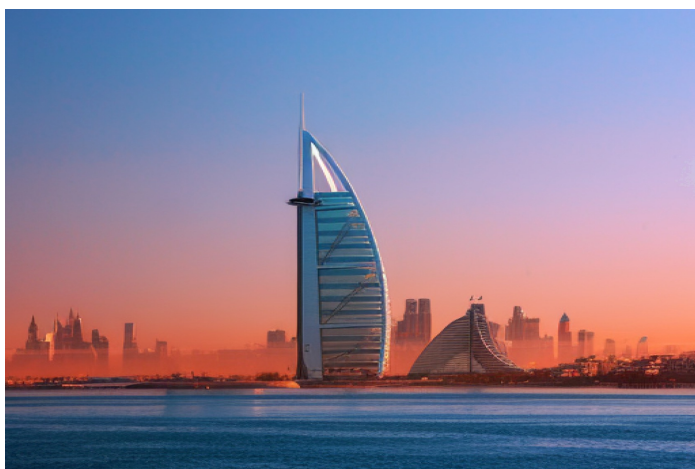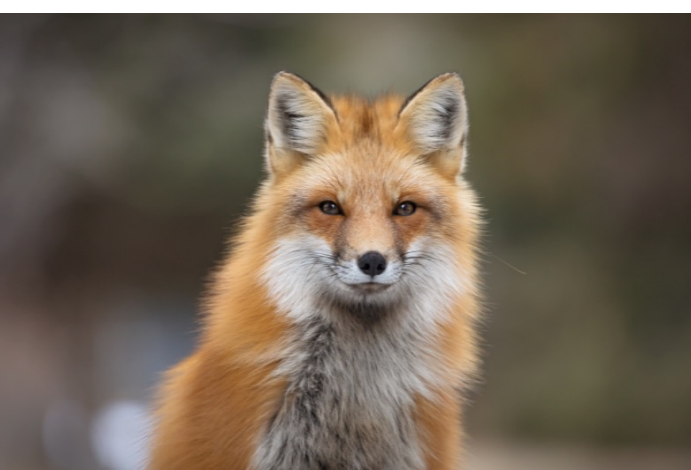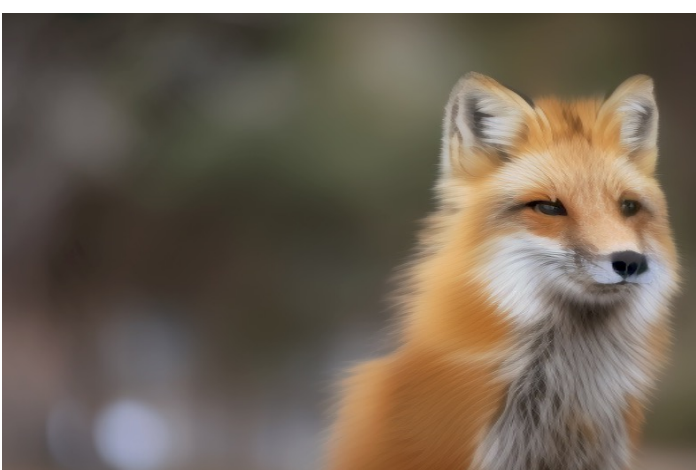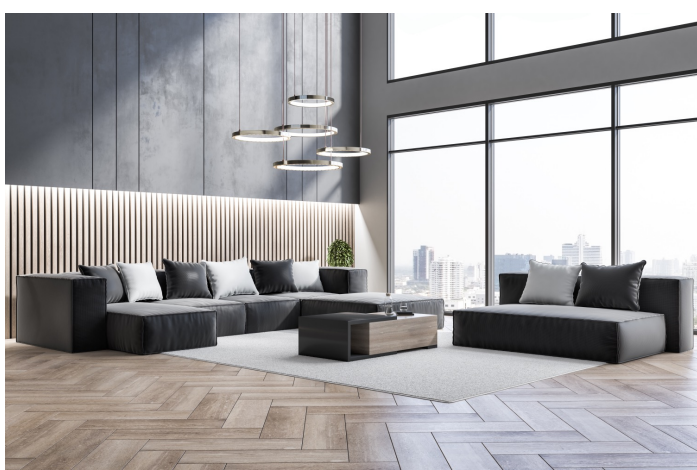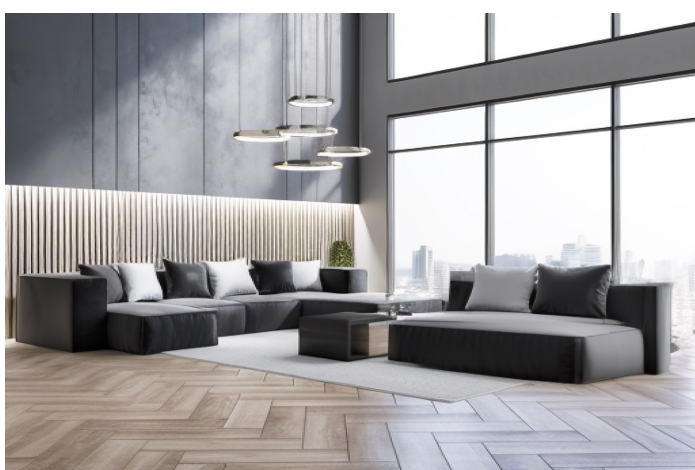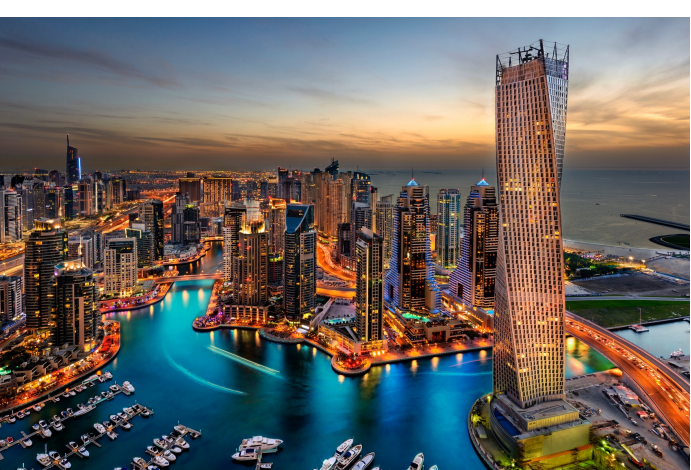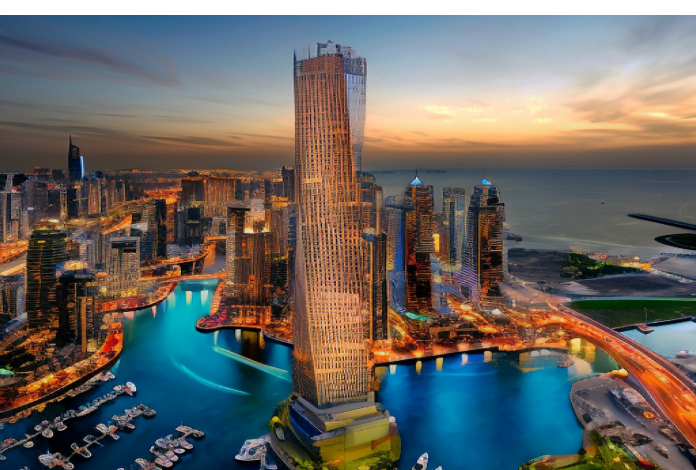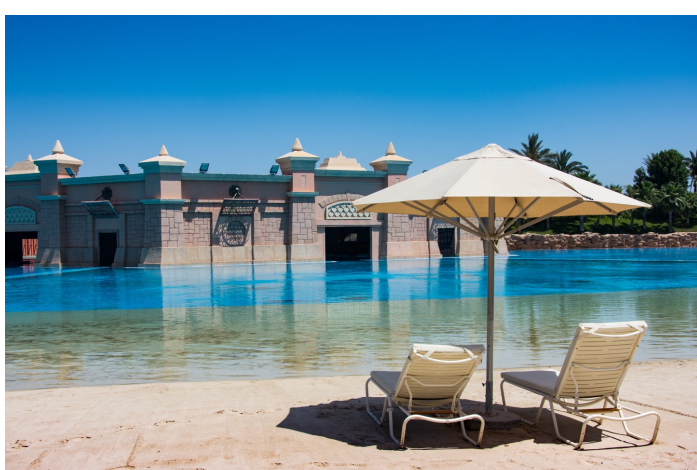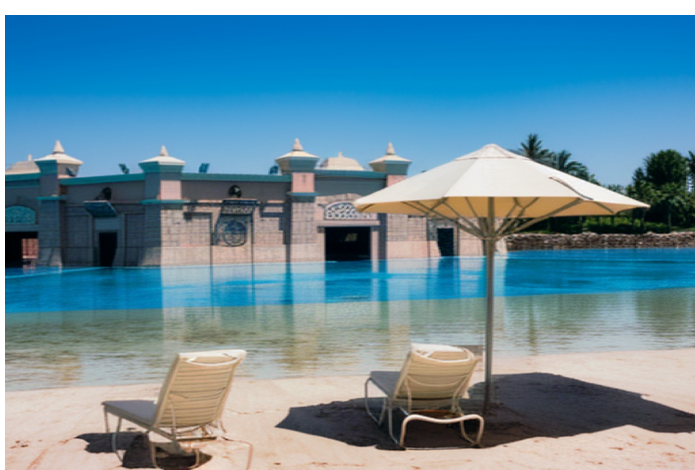

# Removal

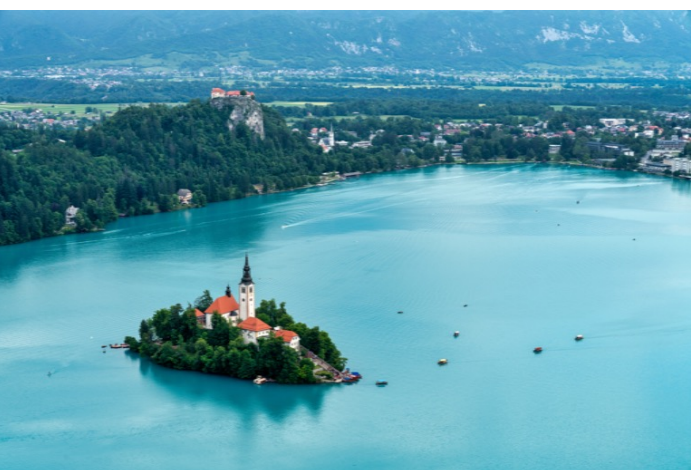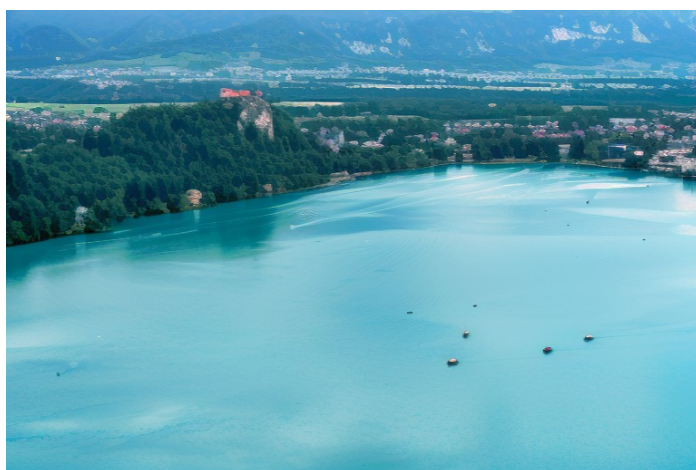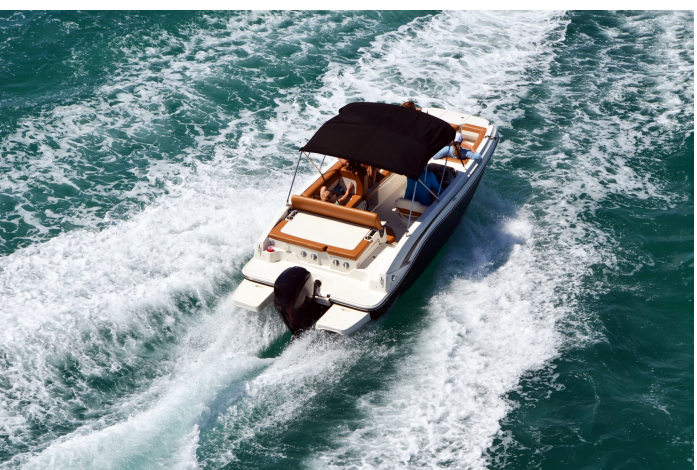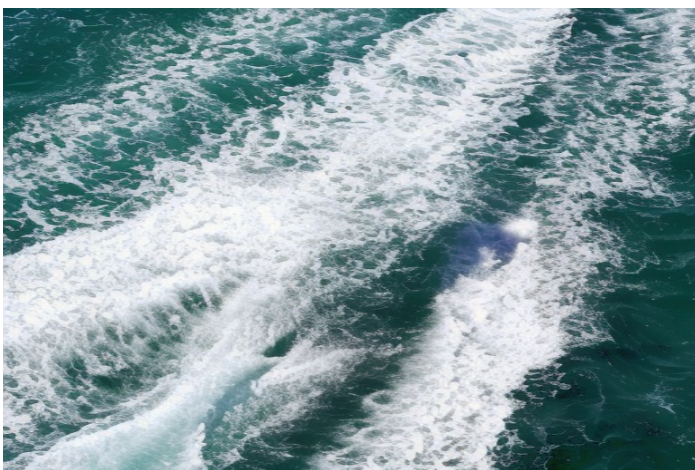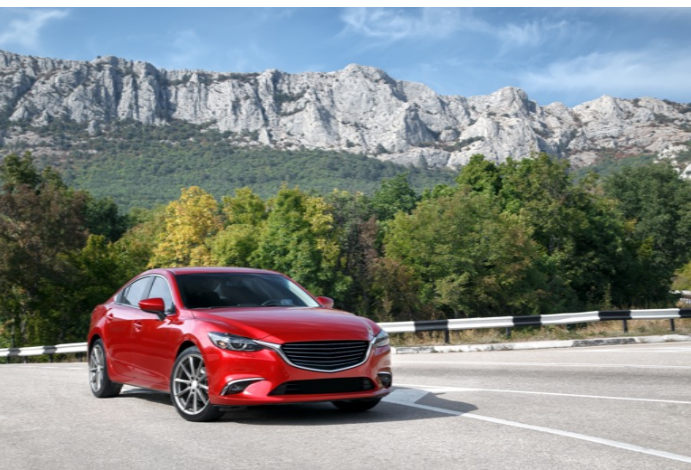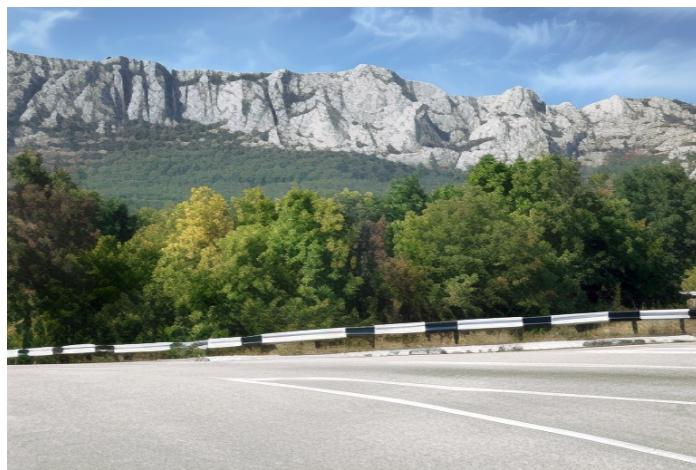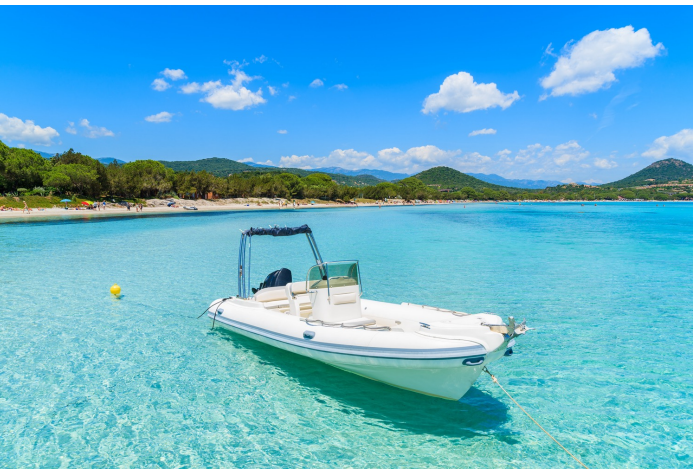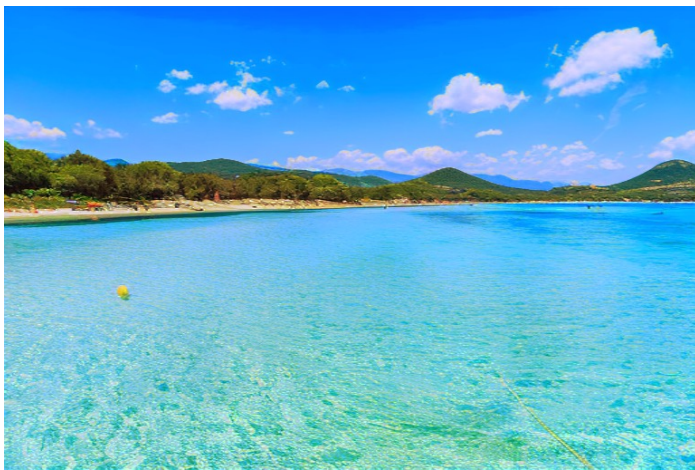



Removal

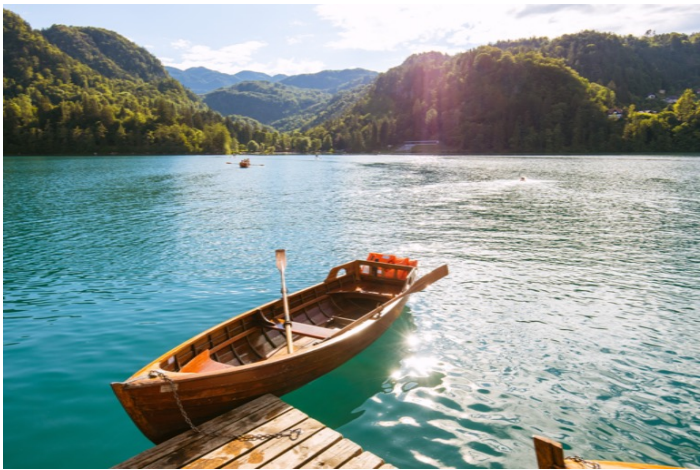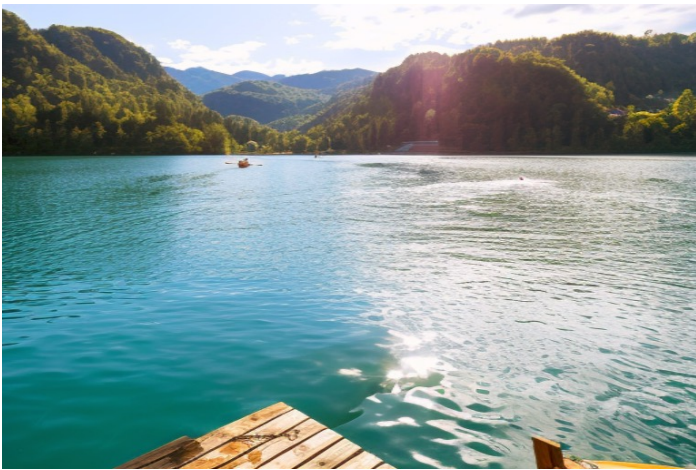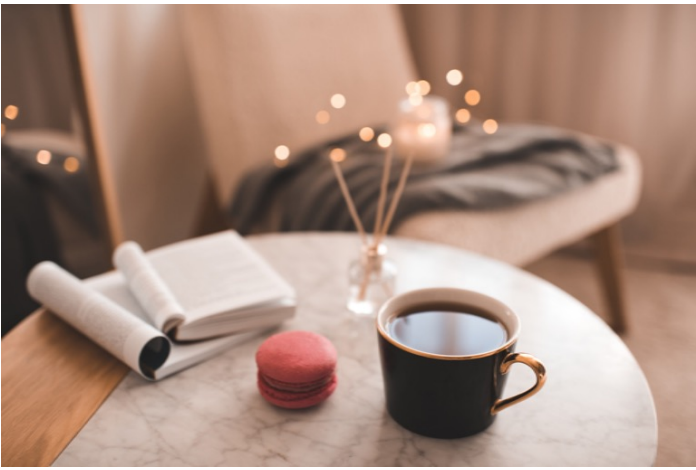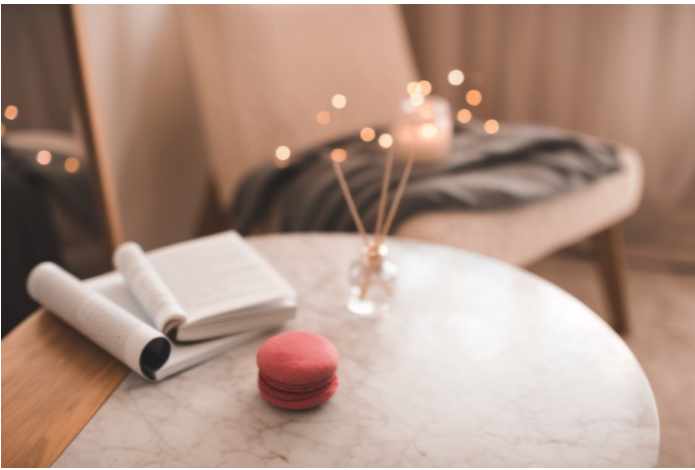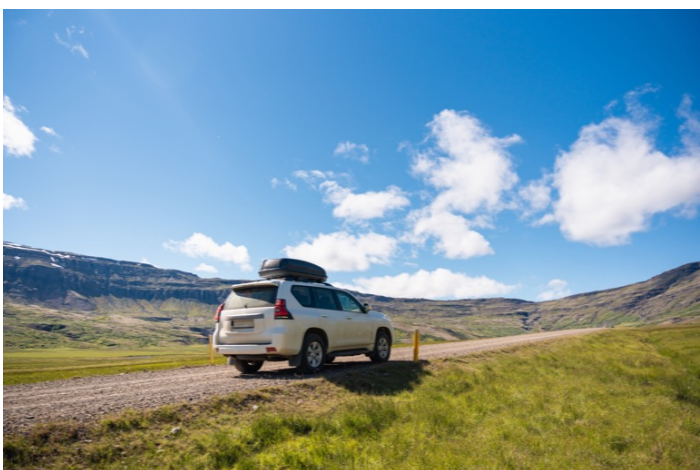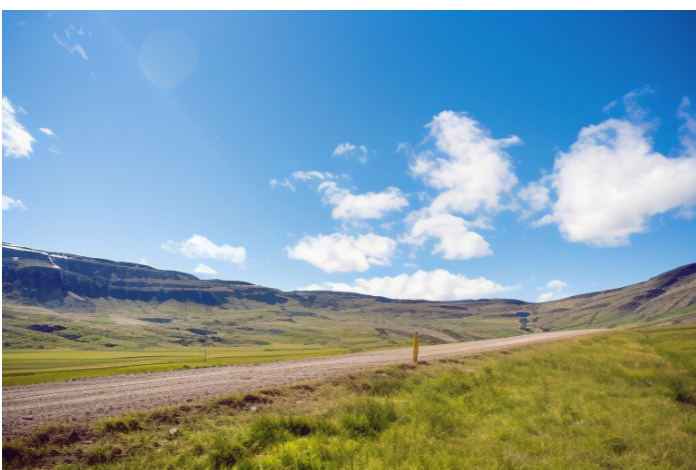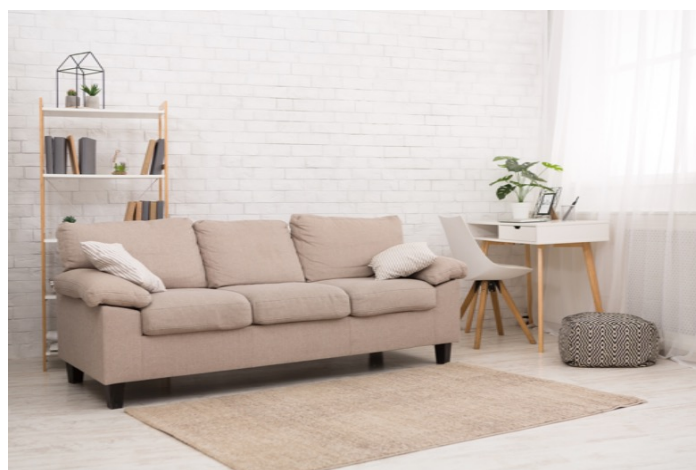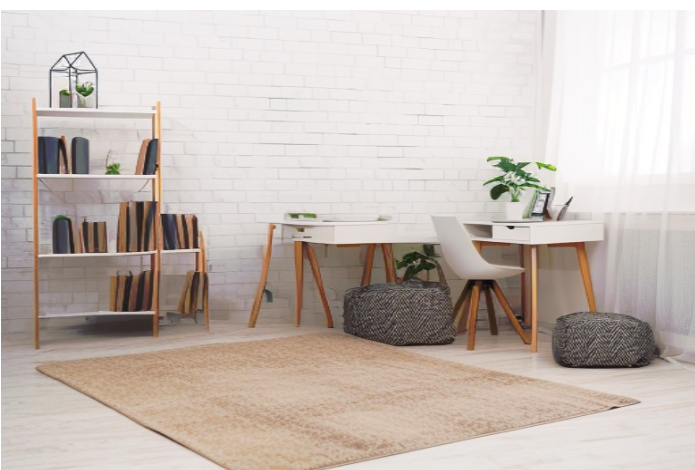

2D Edits

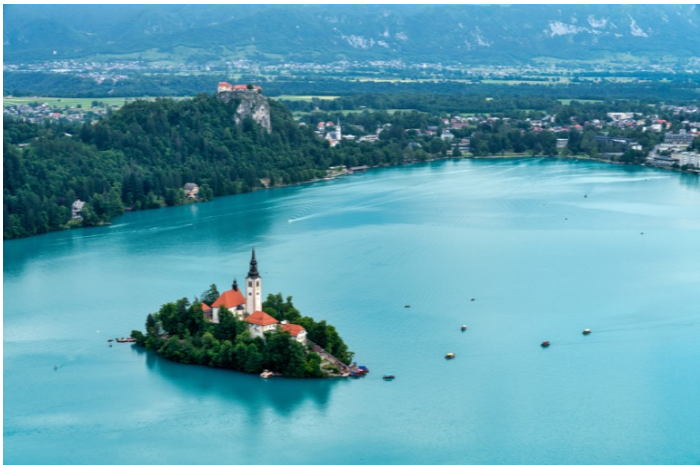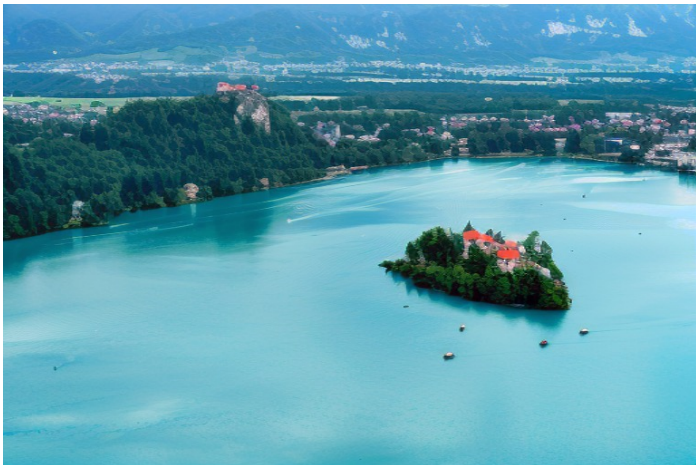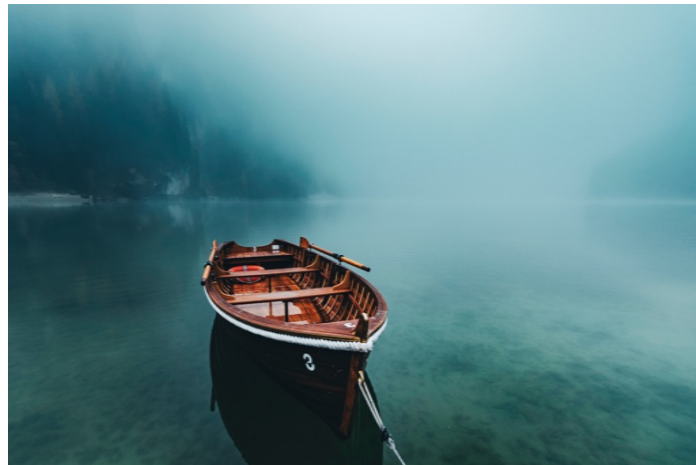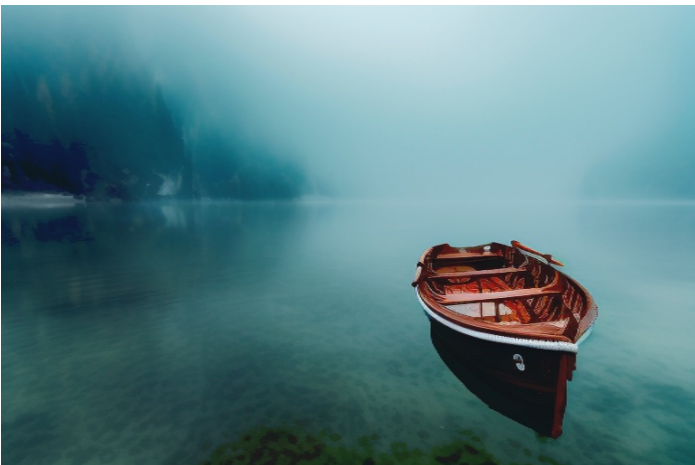

3D Edits

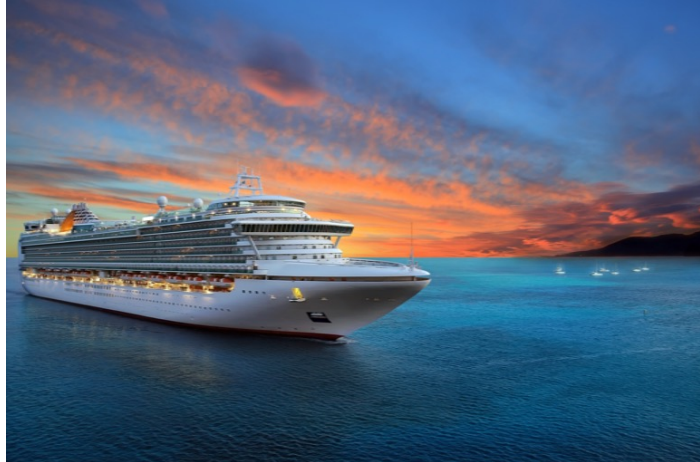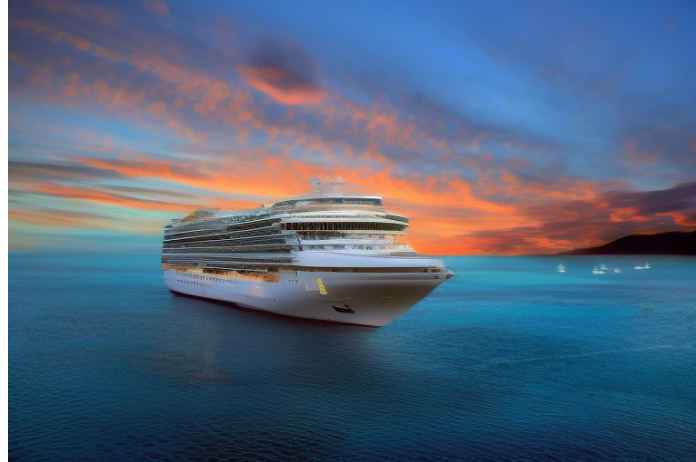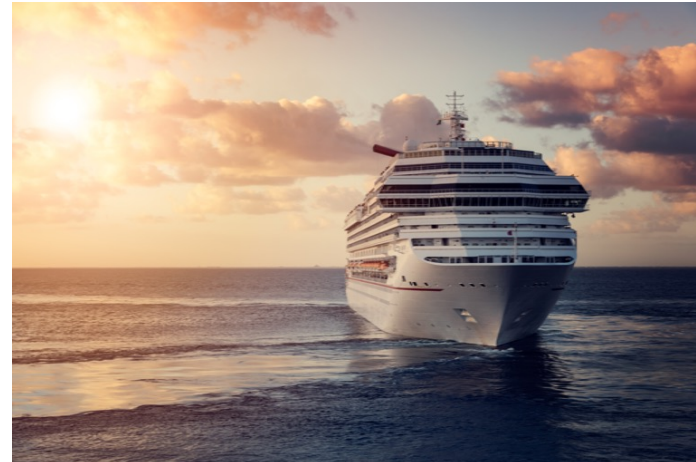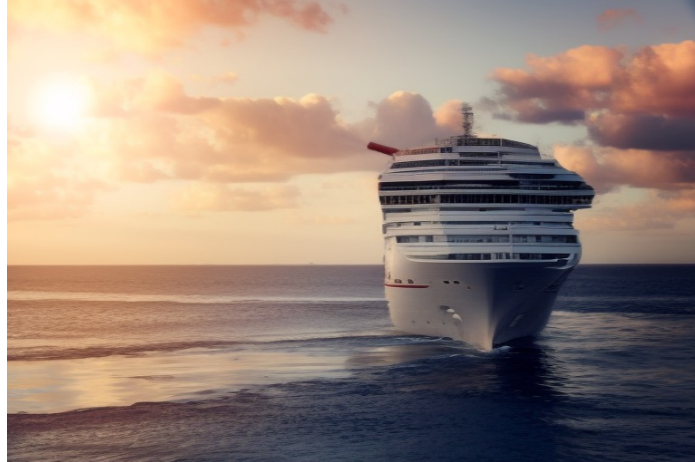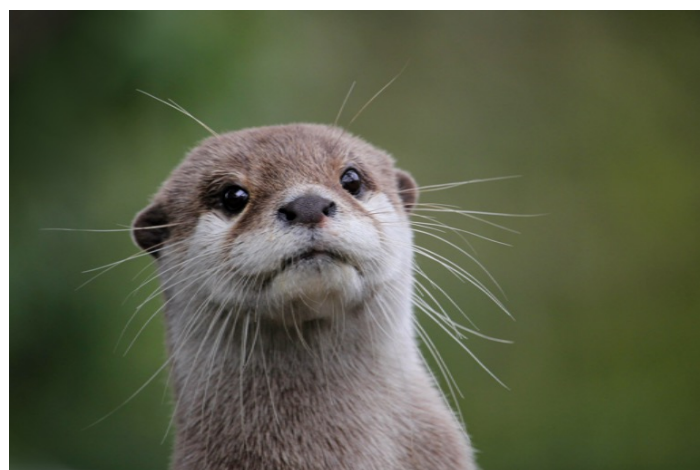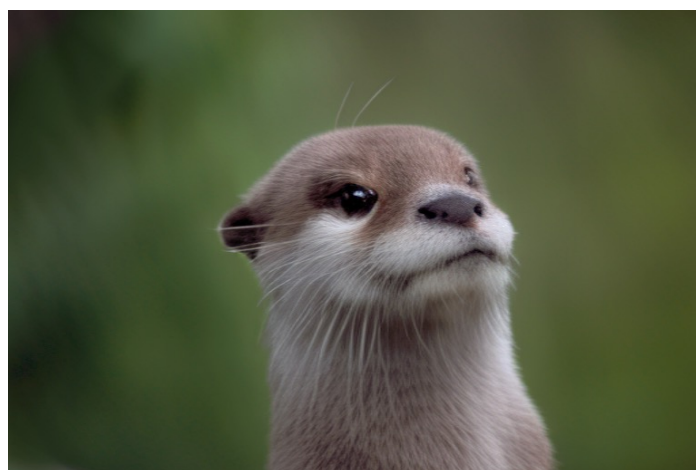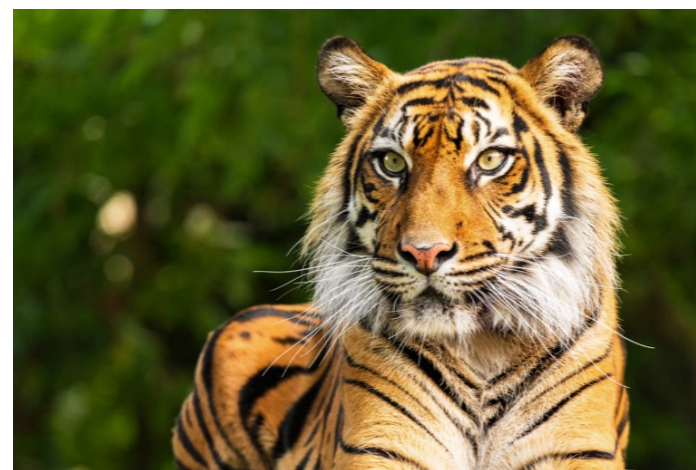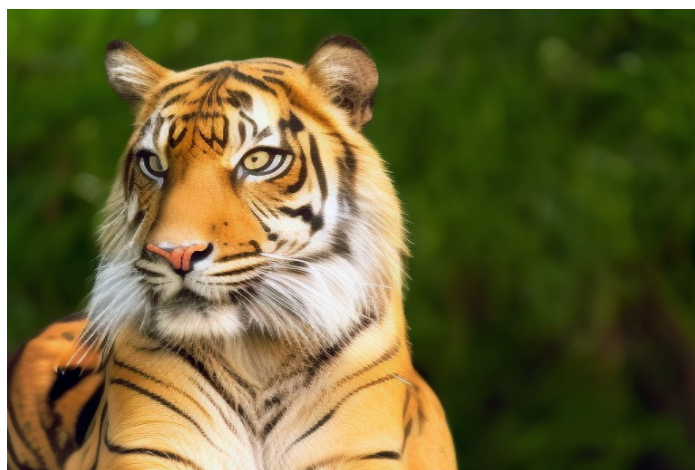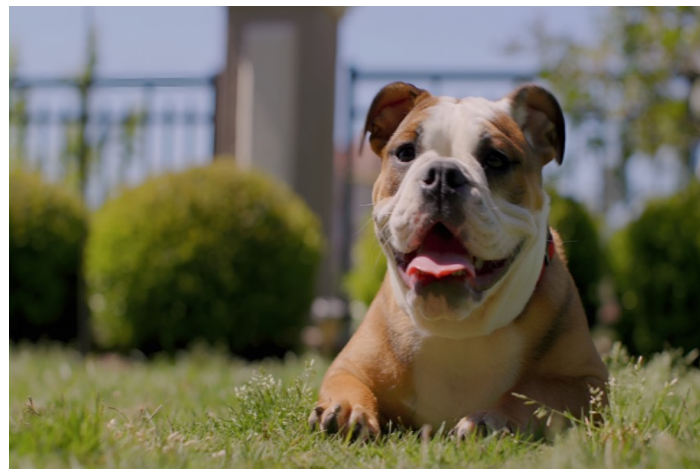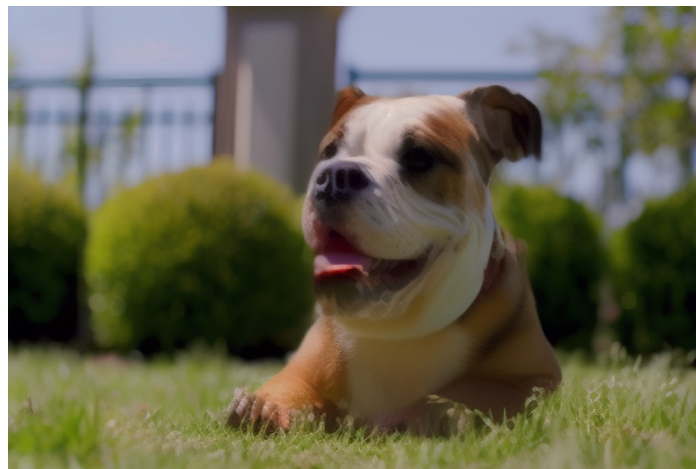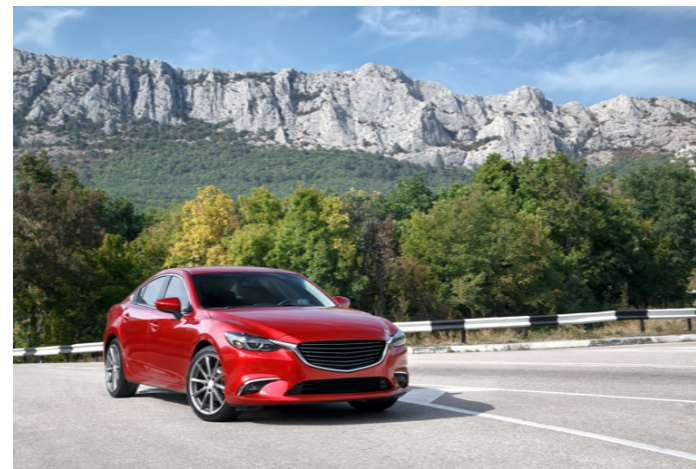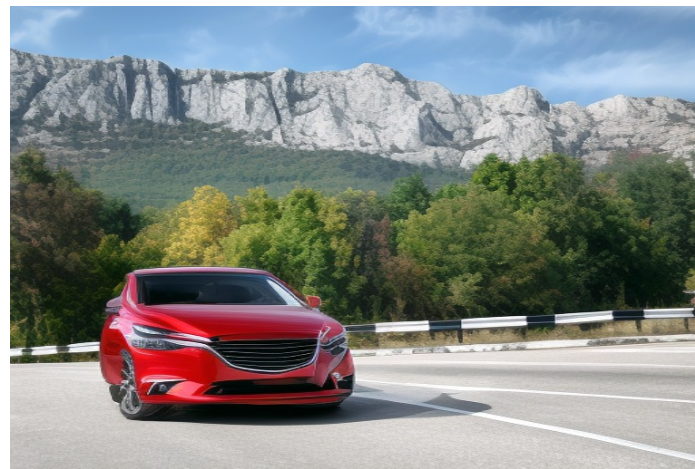

Scaling

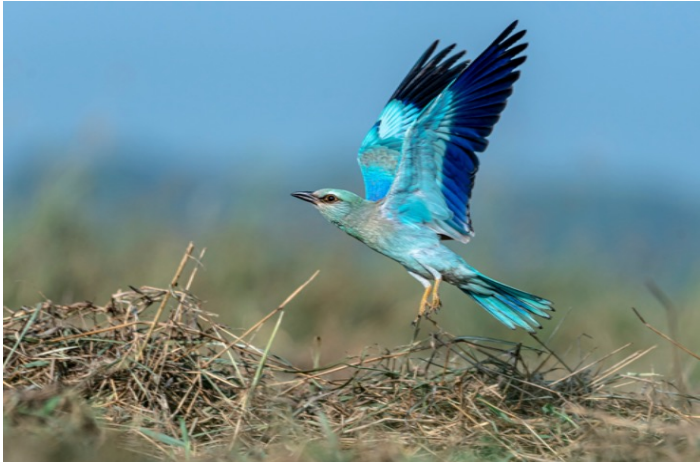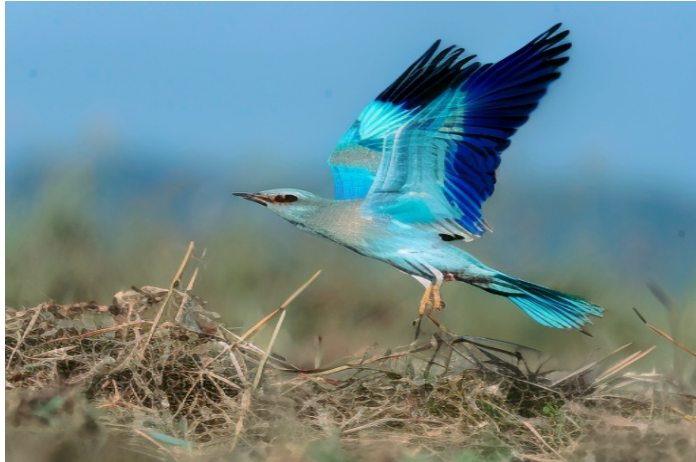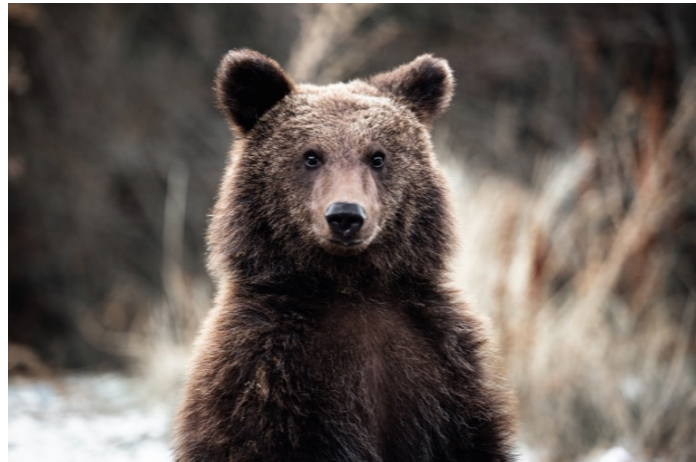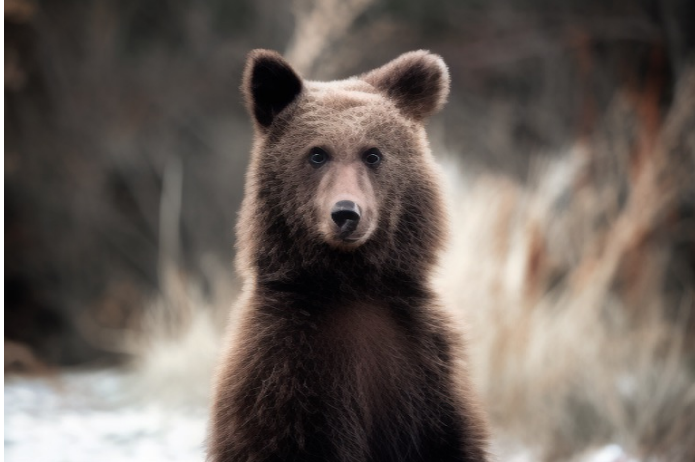



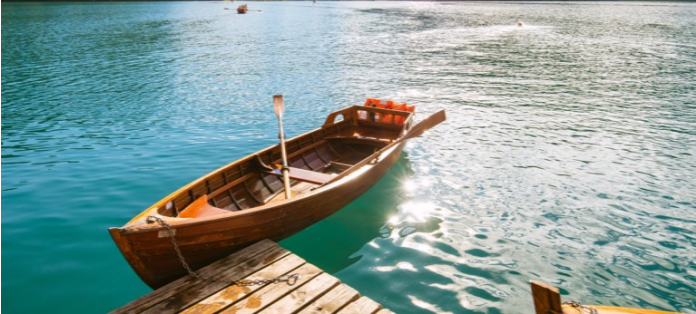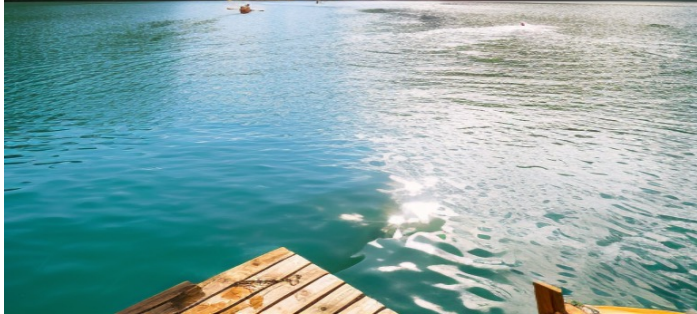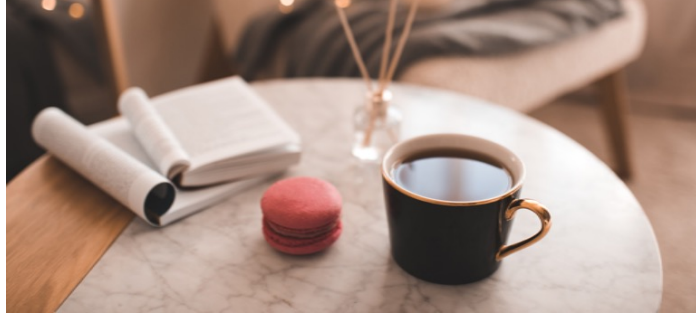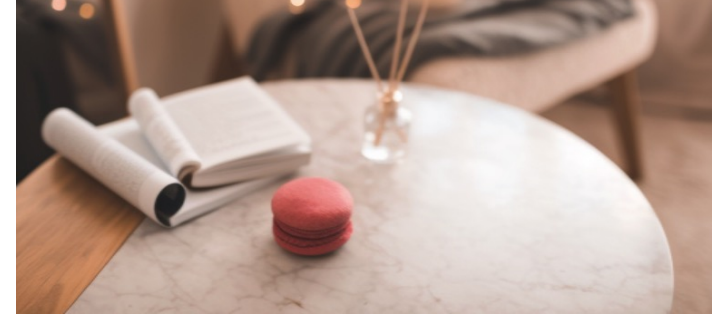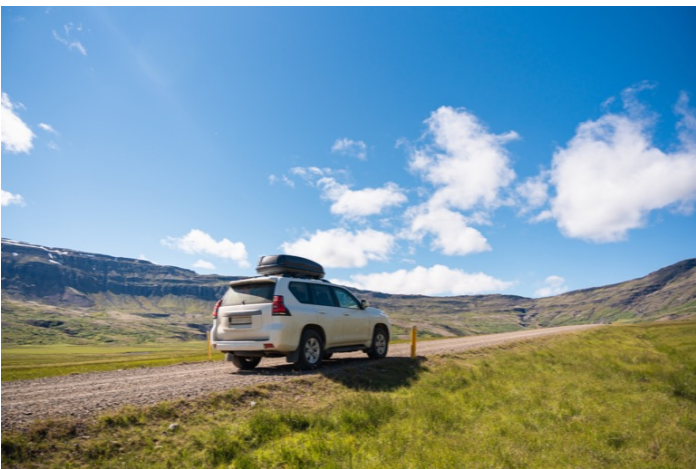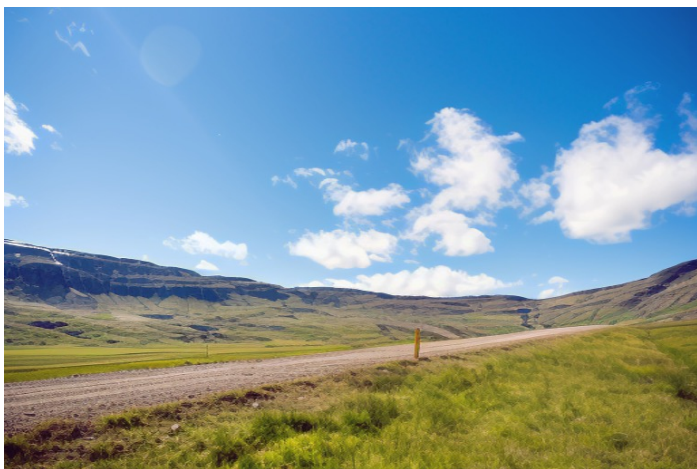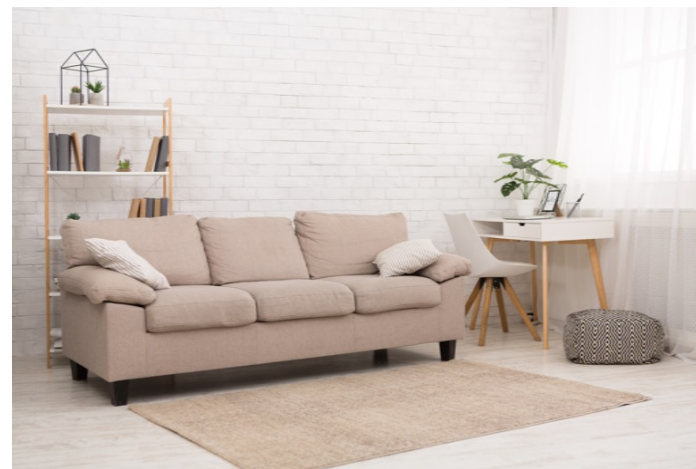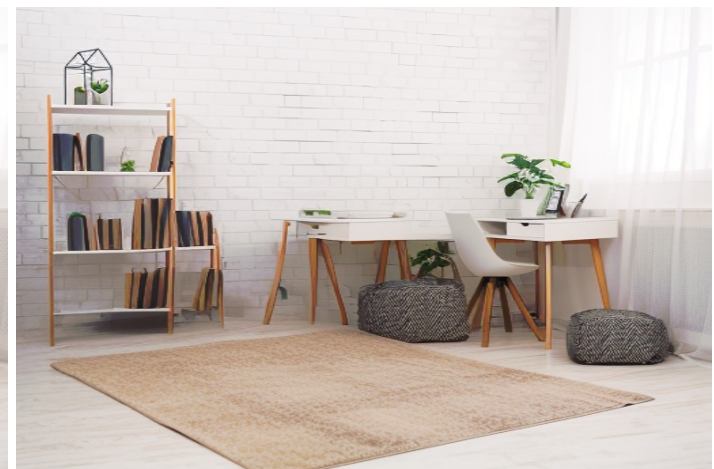

## 2D Edits

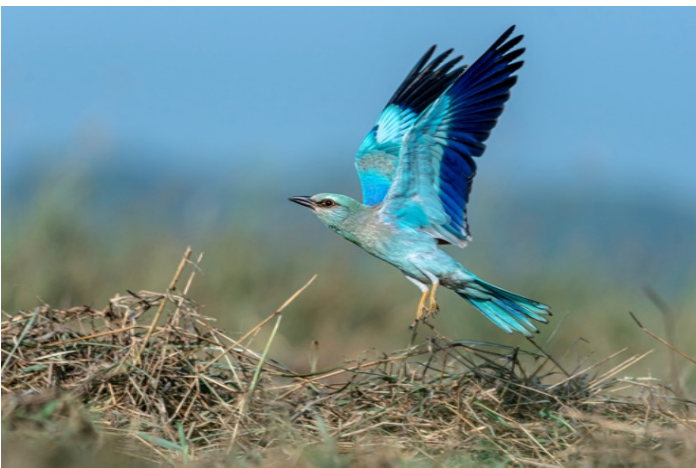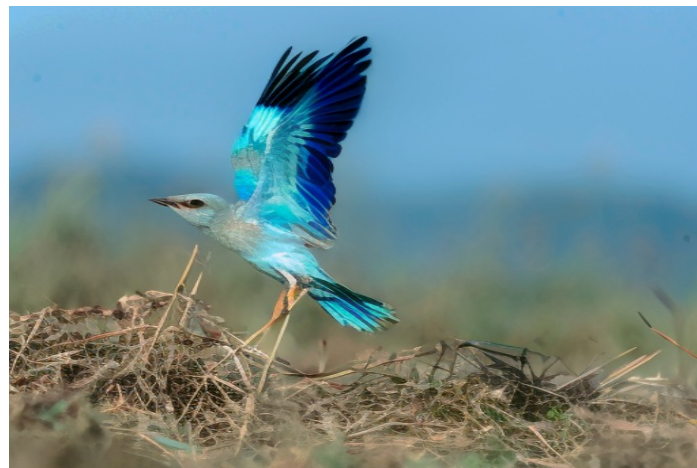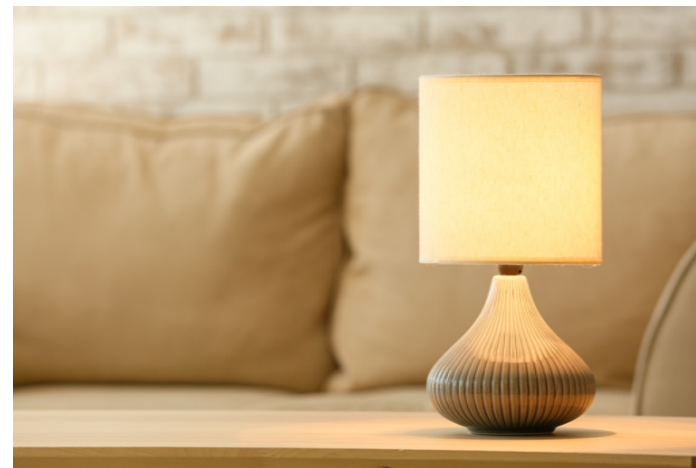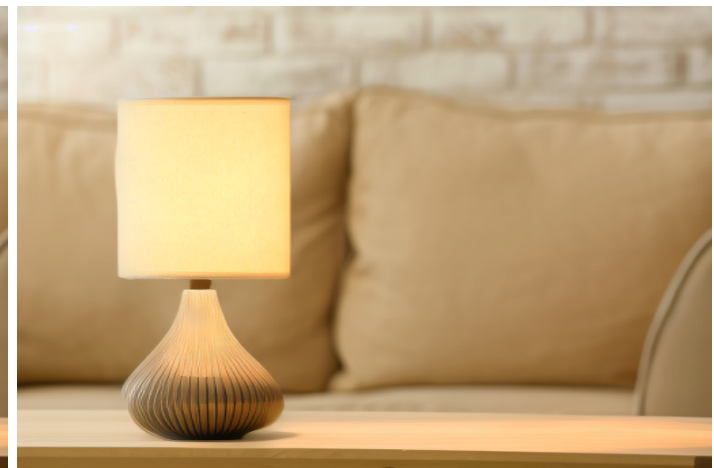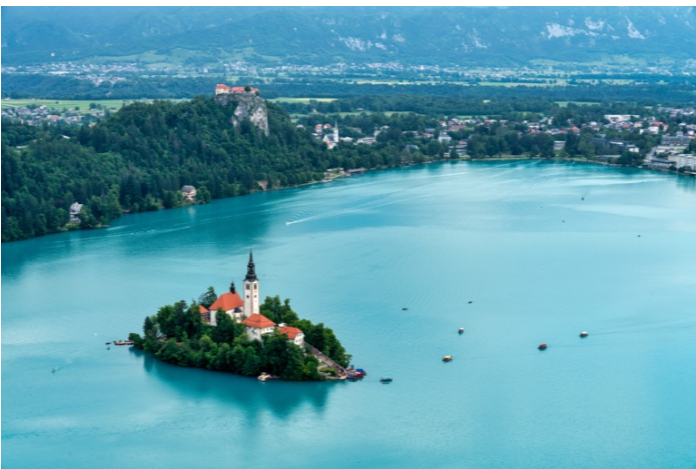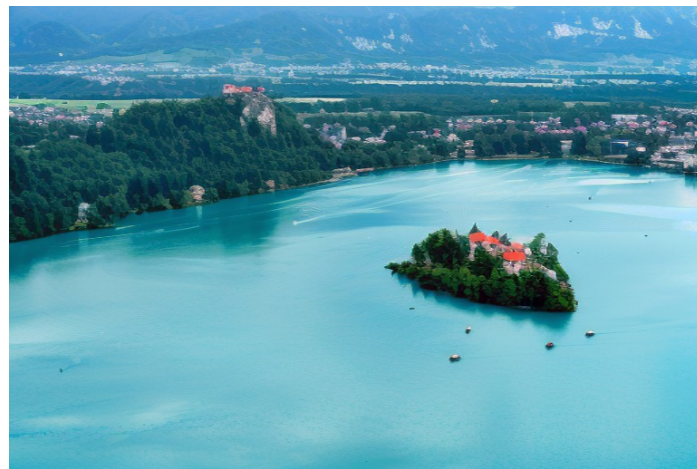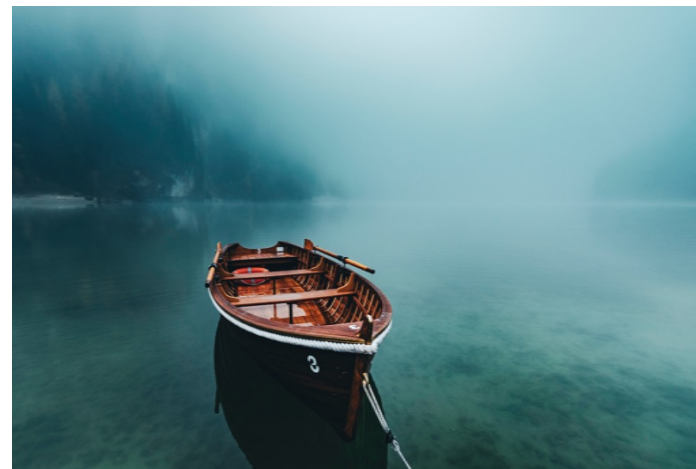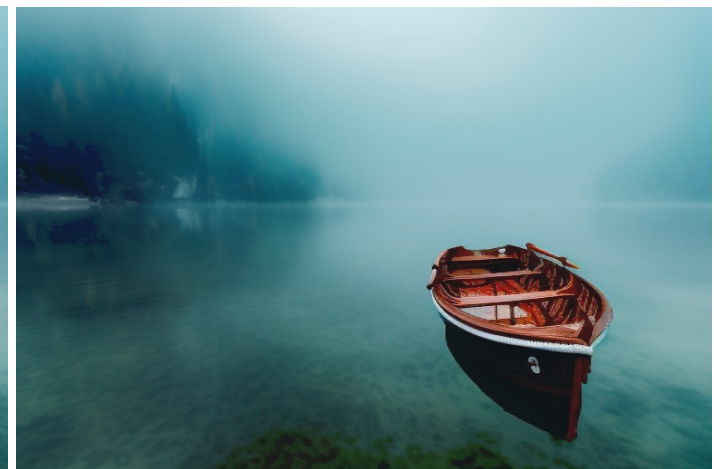

## 3D Edits

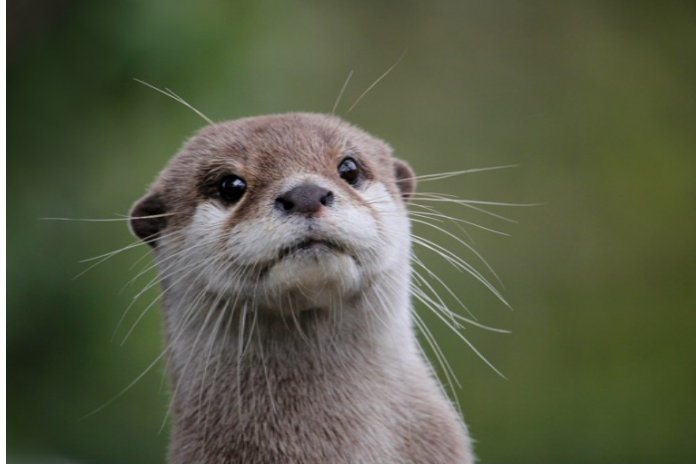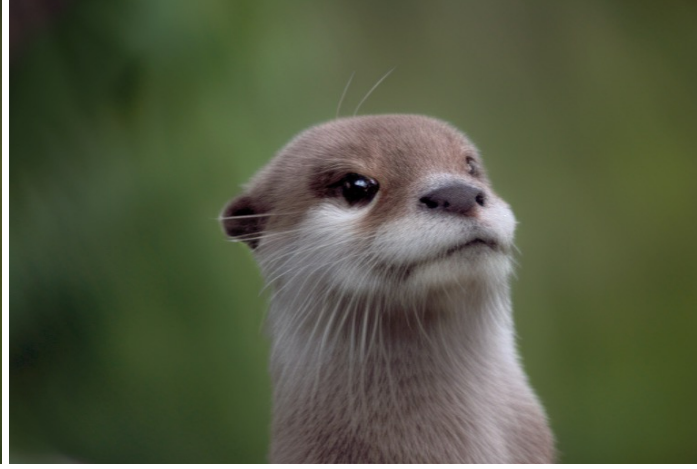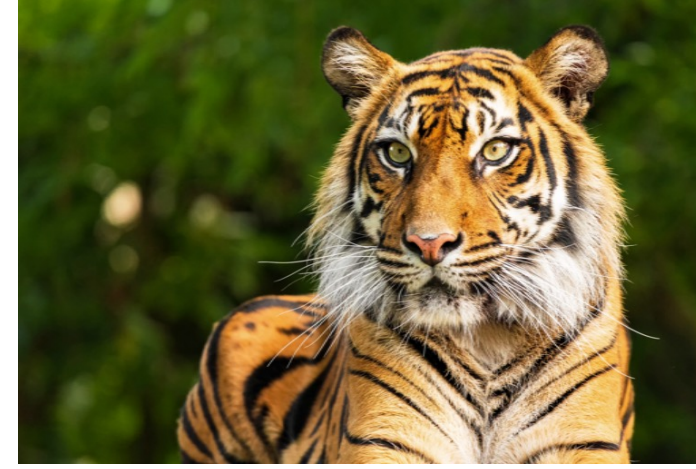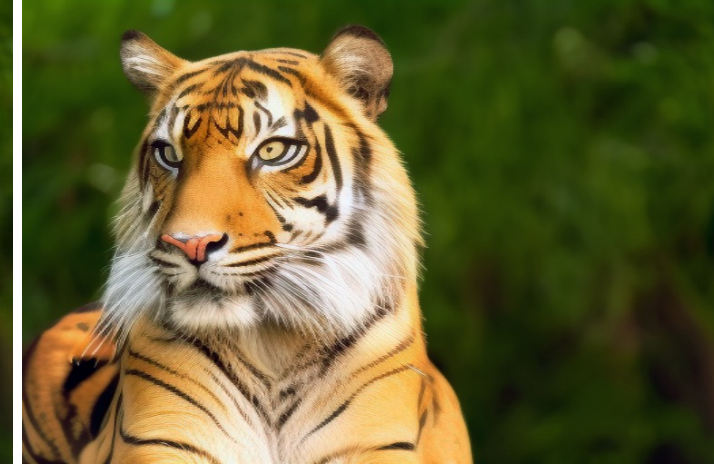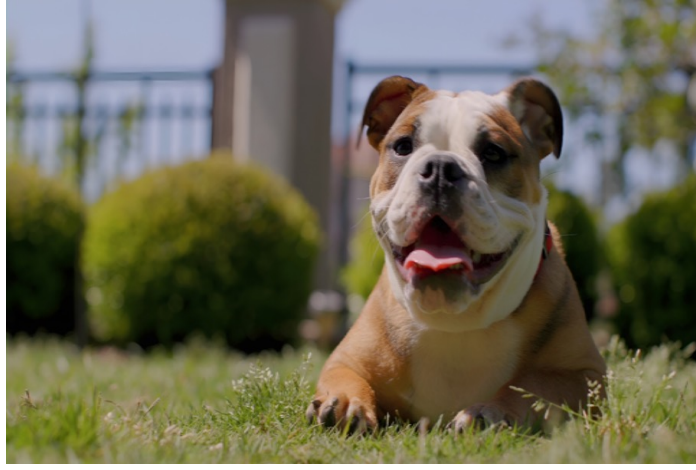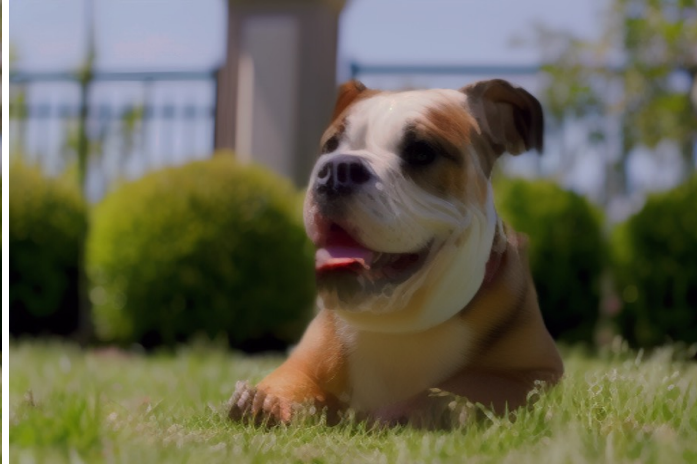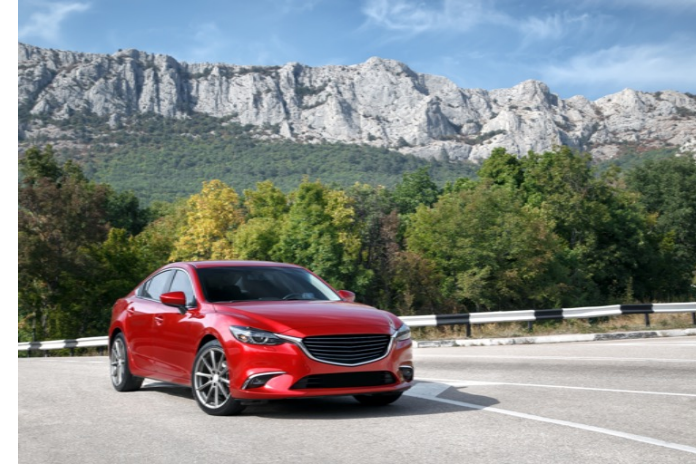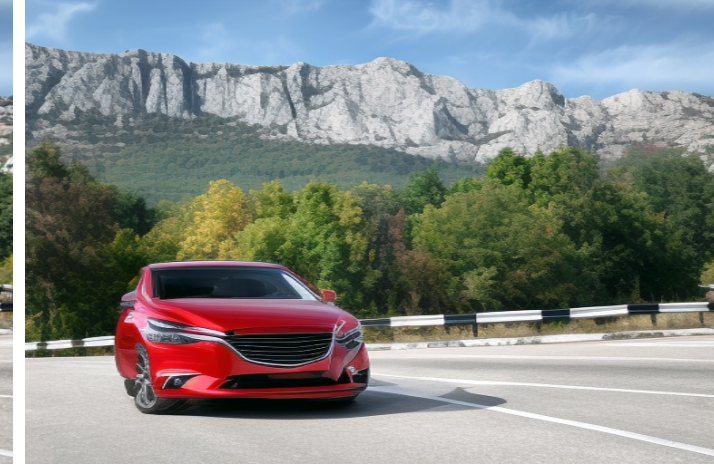

## Scaling

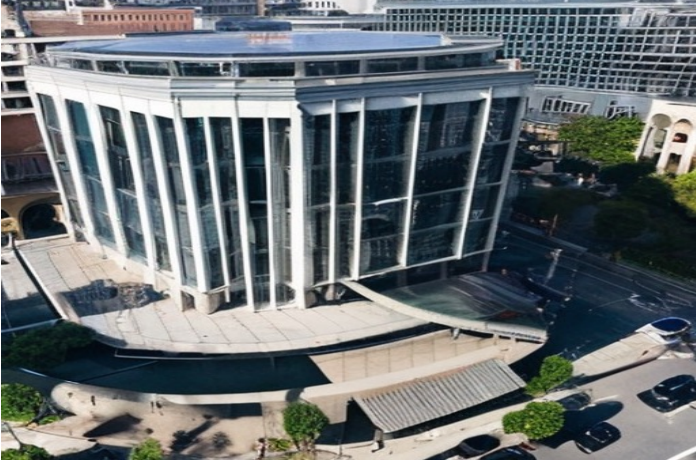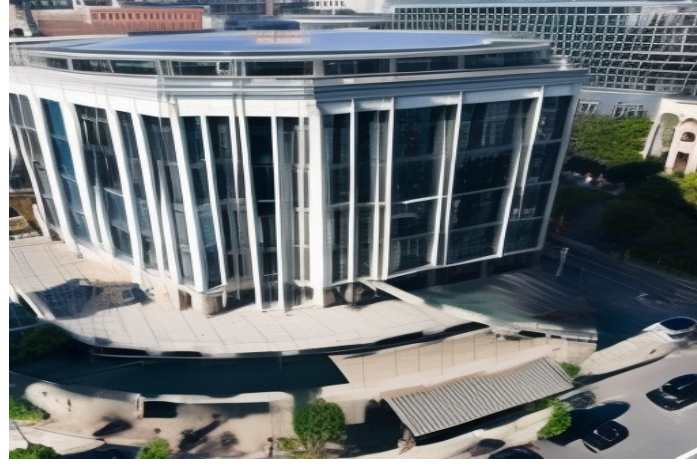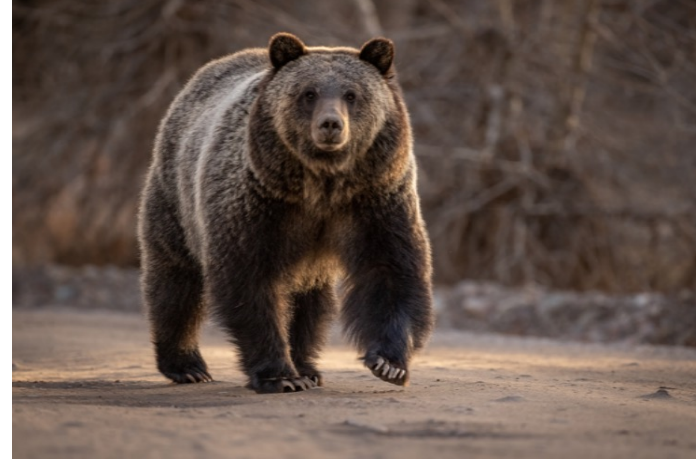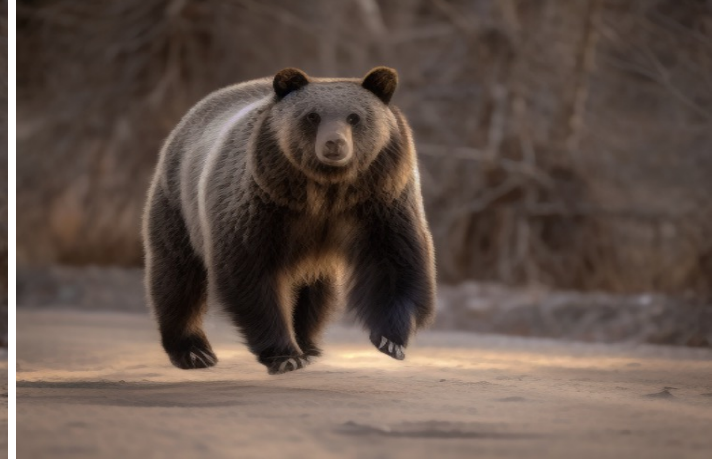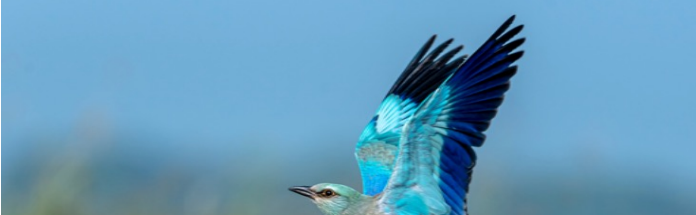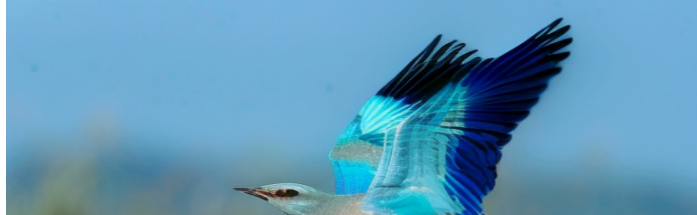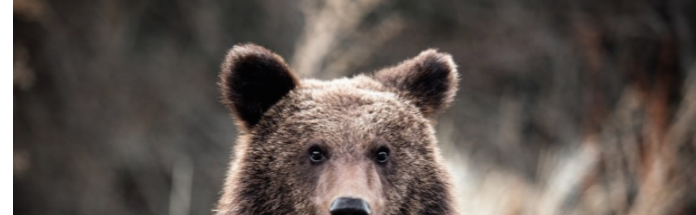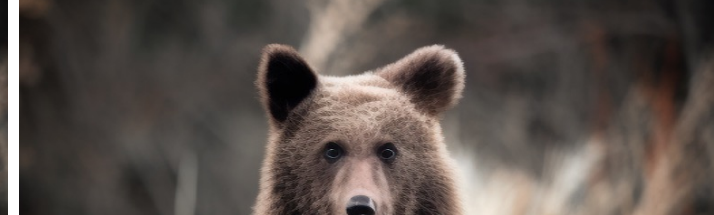



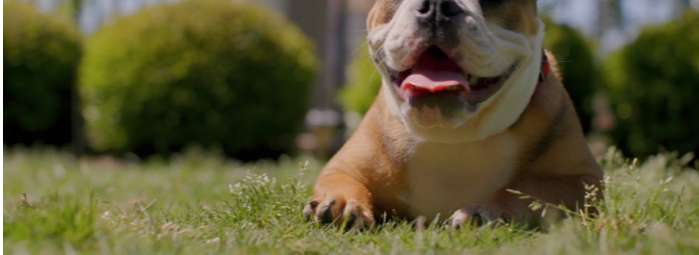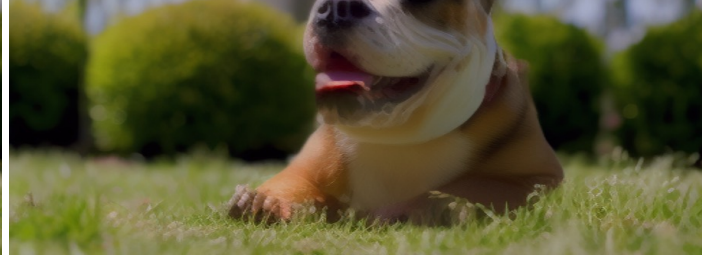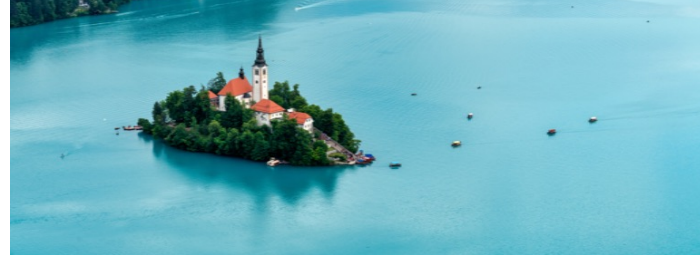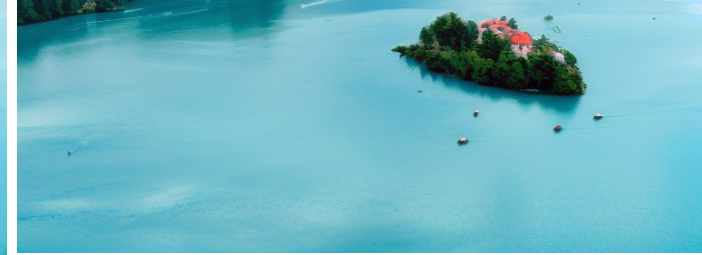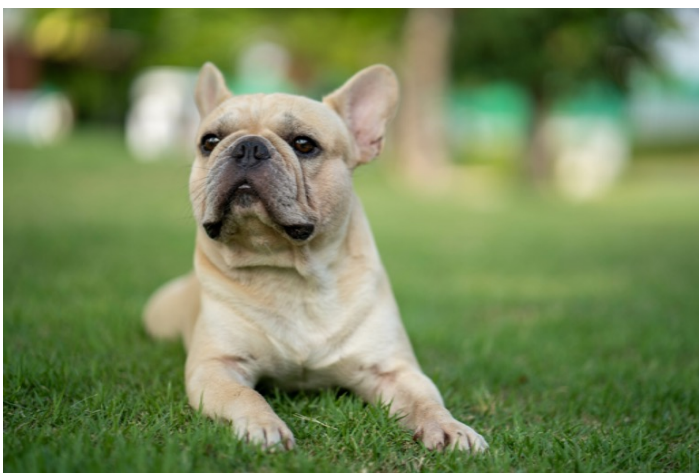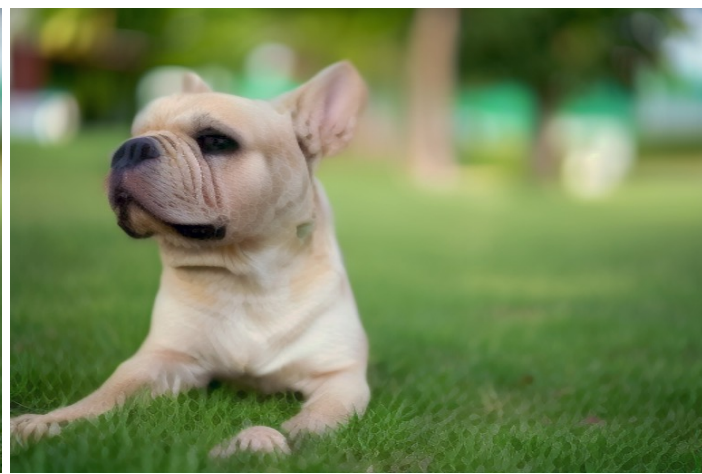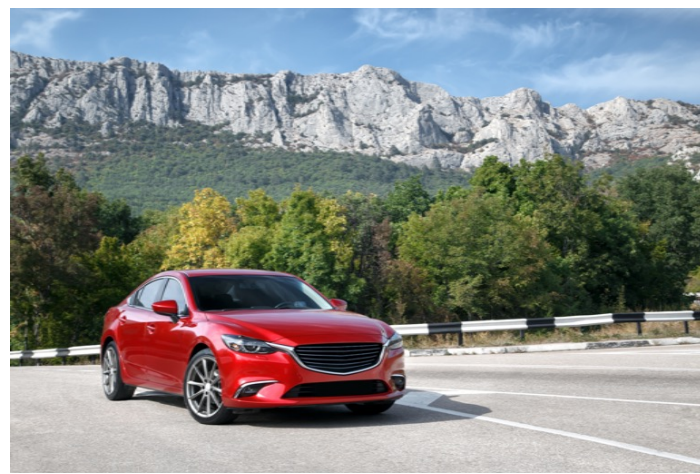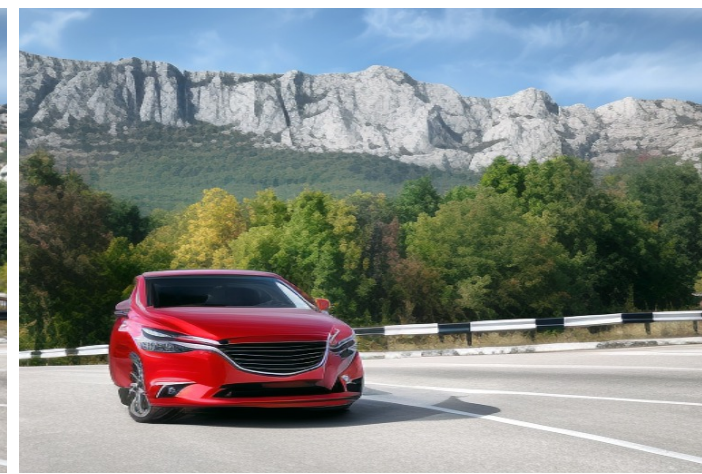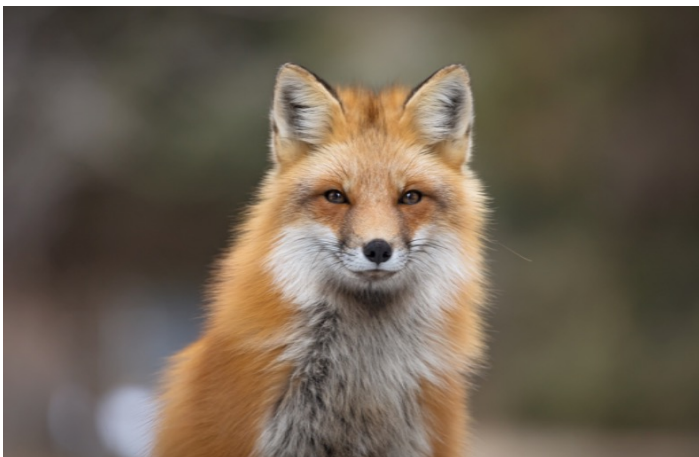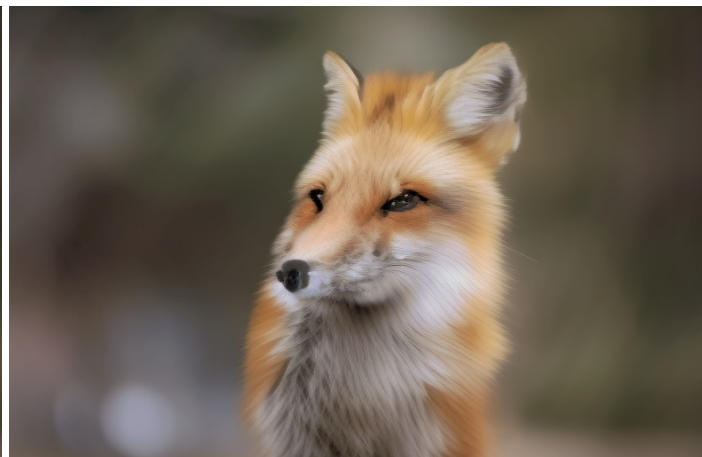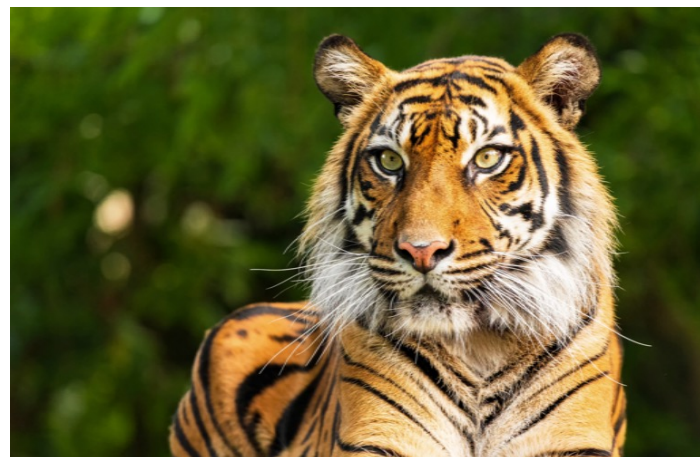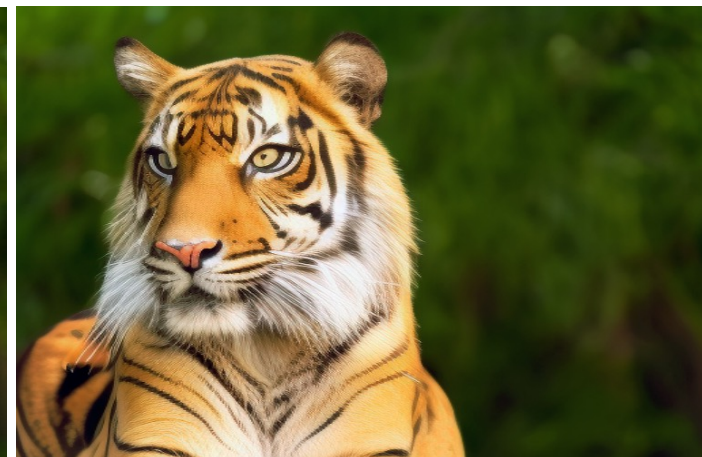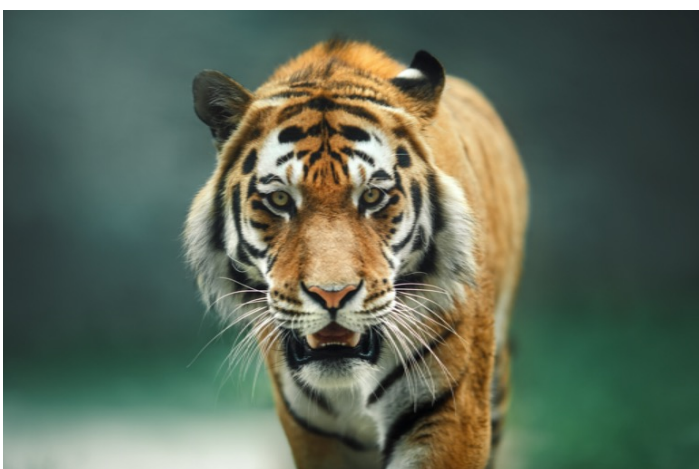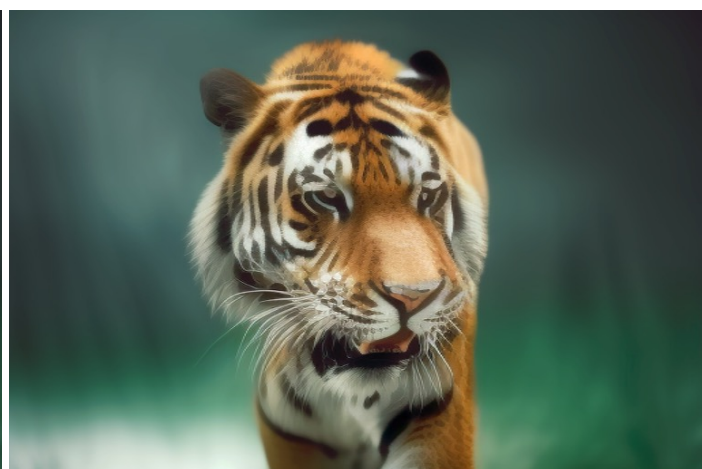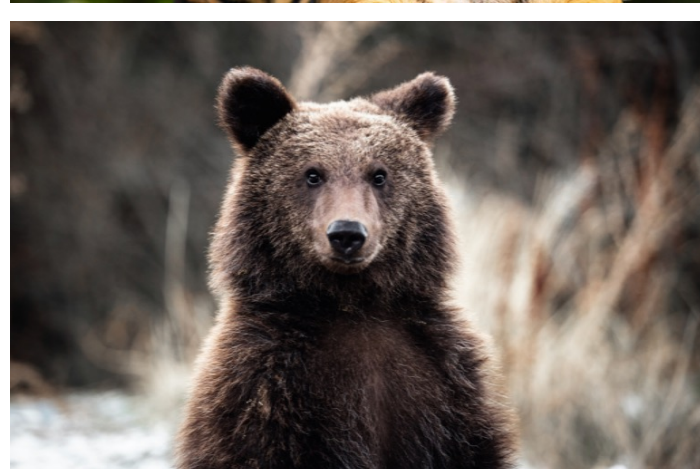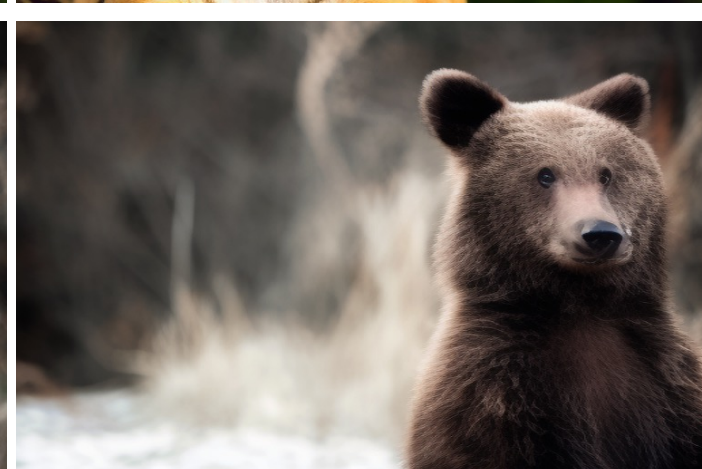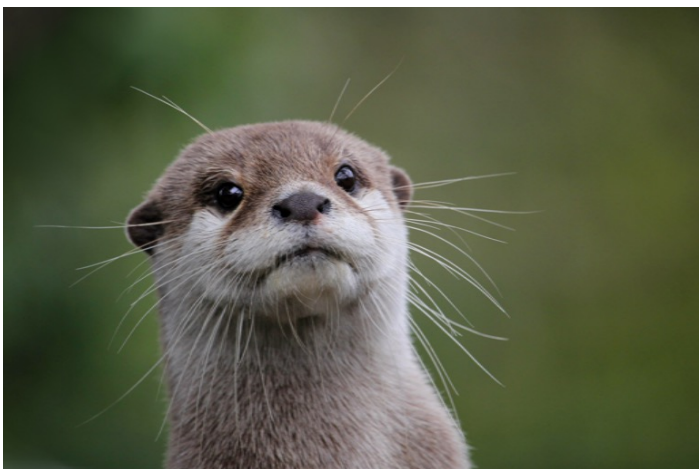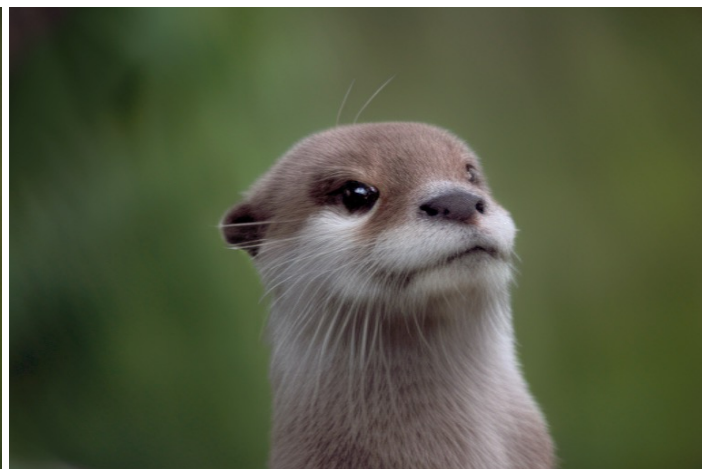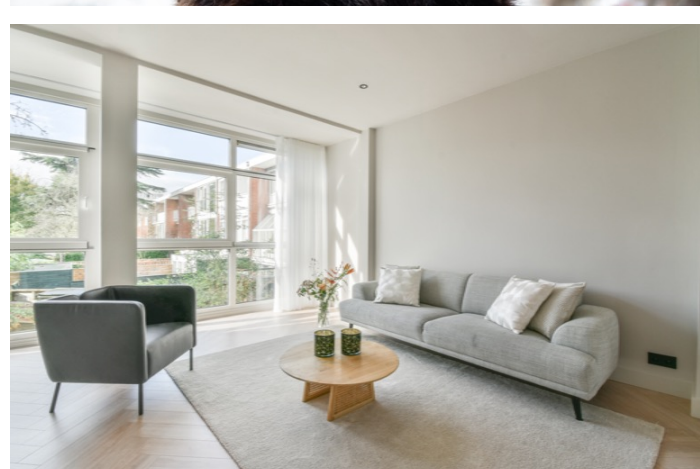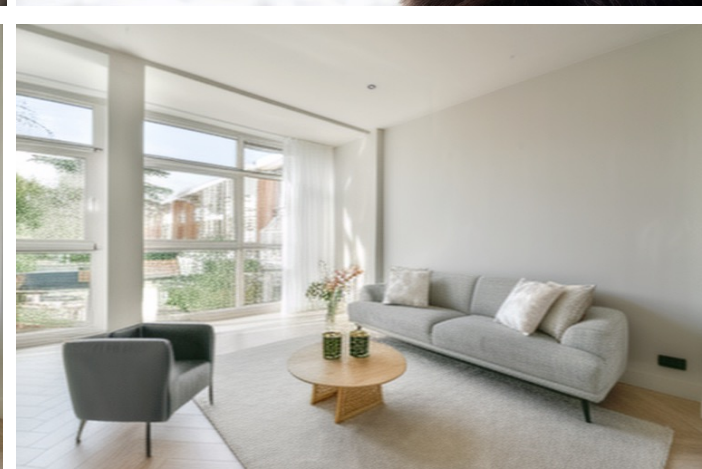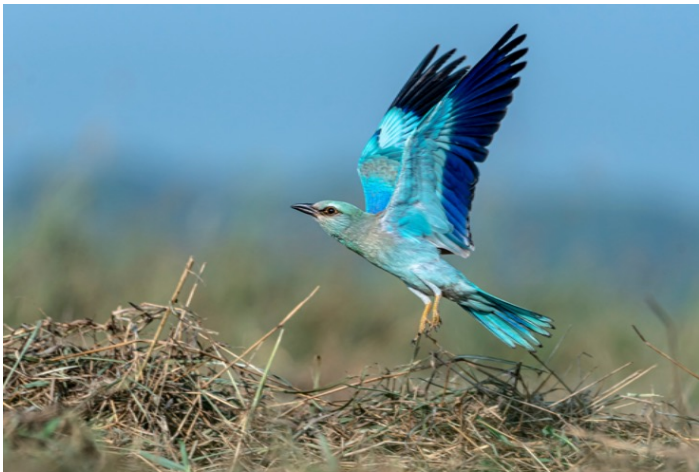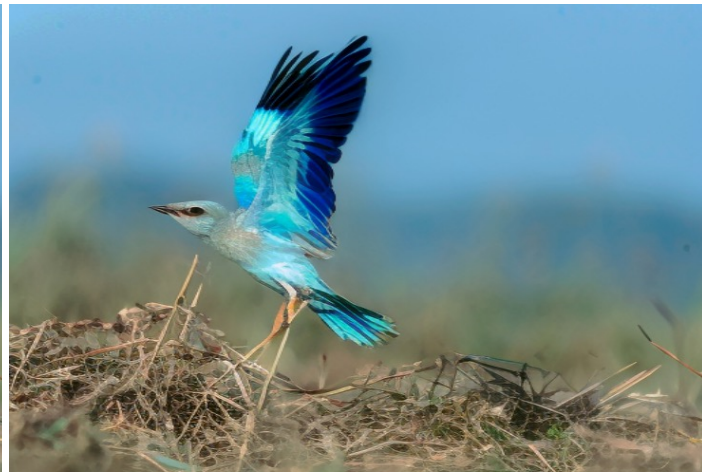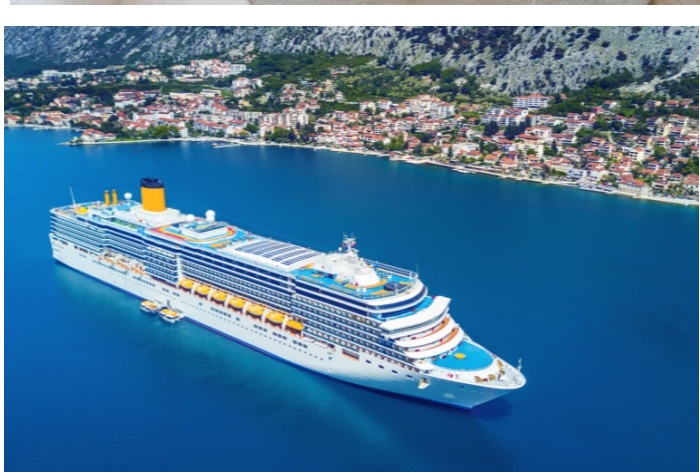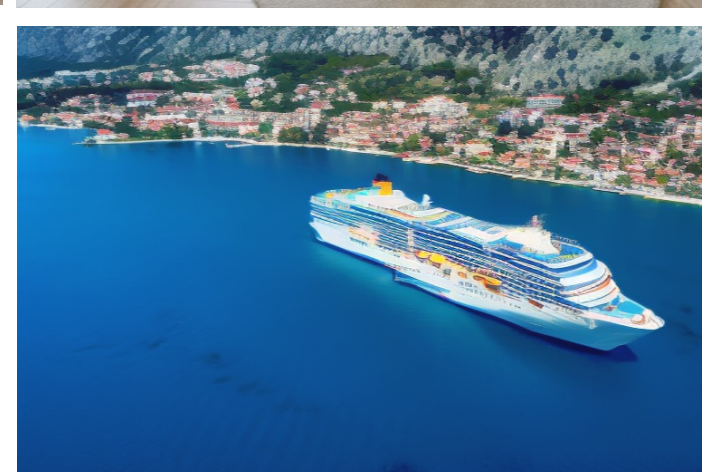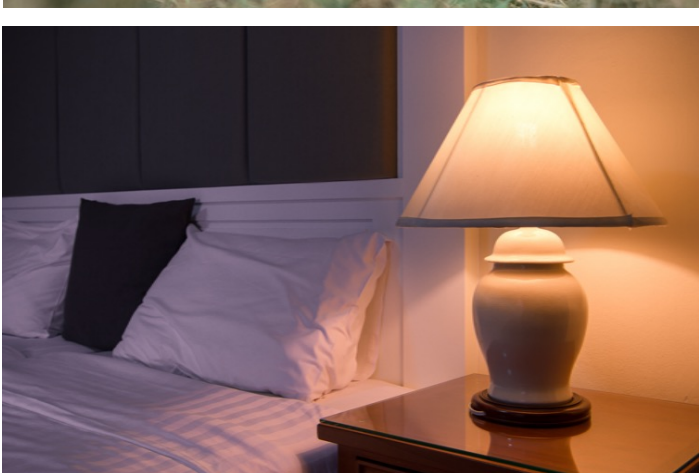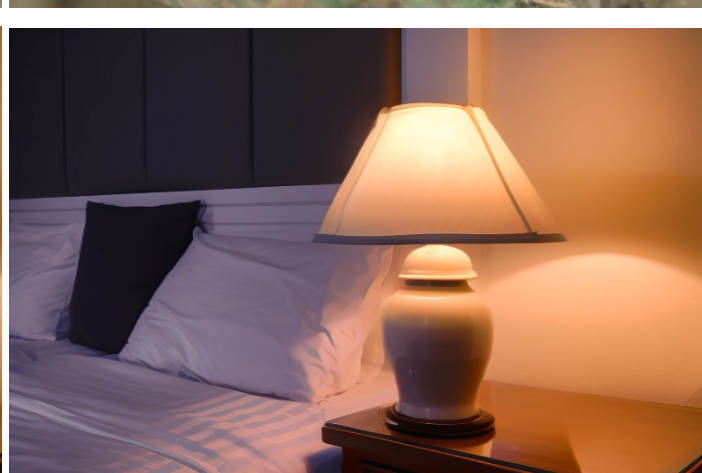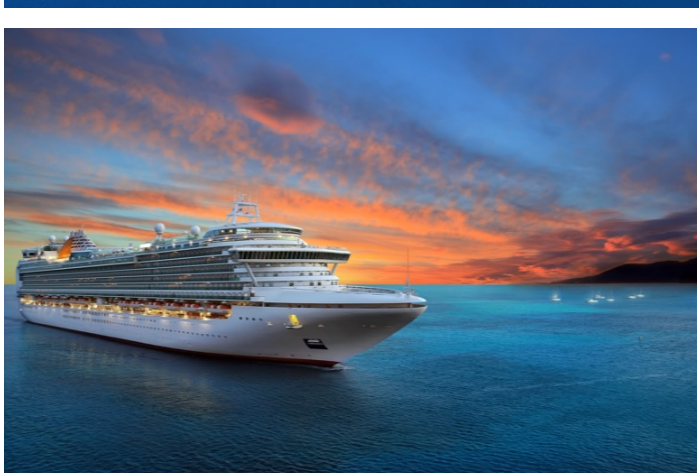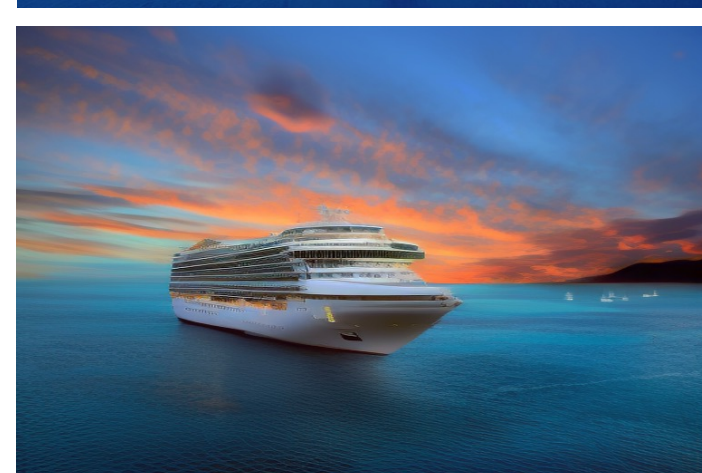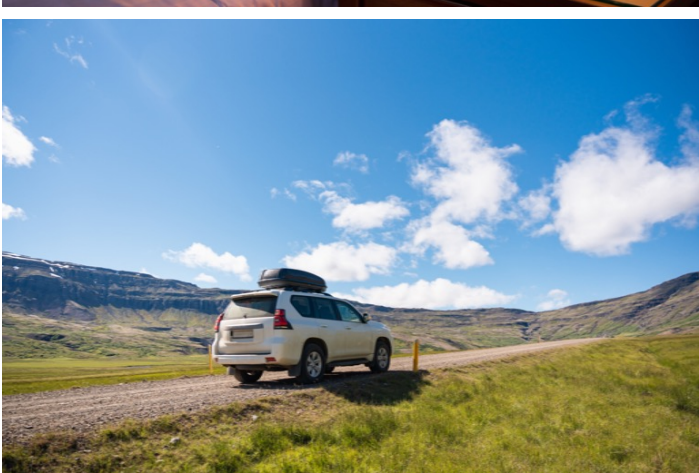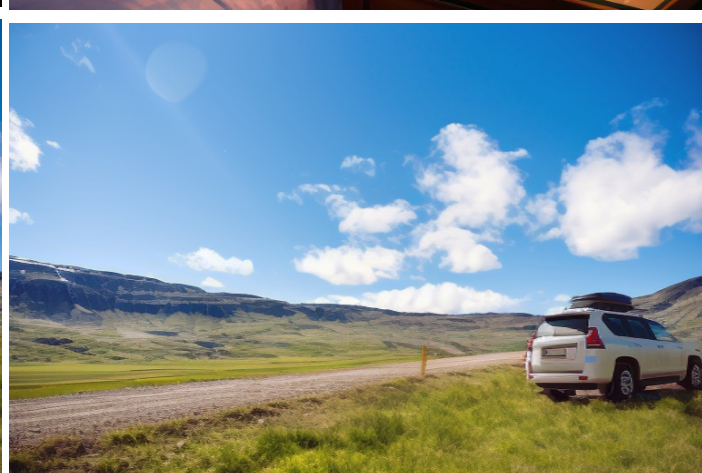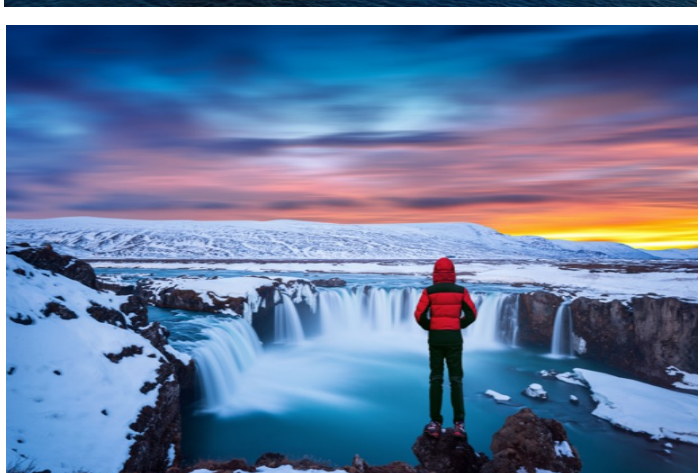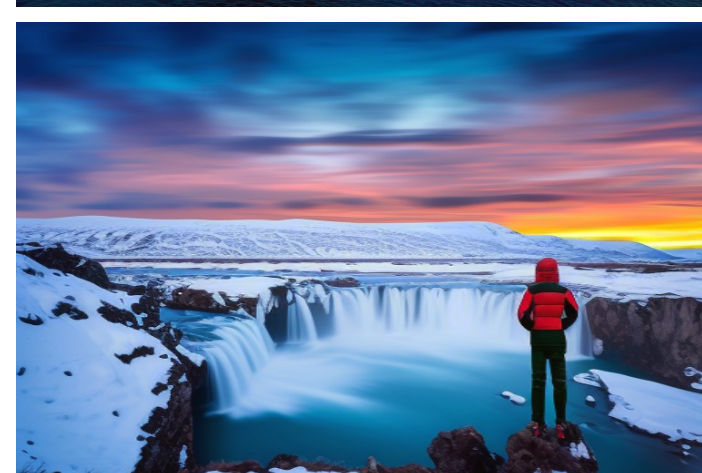



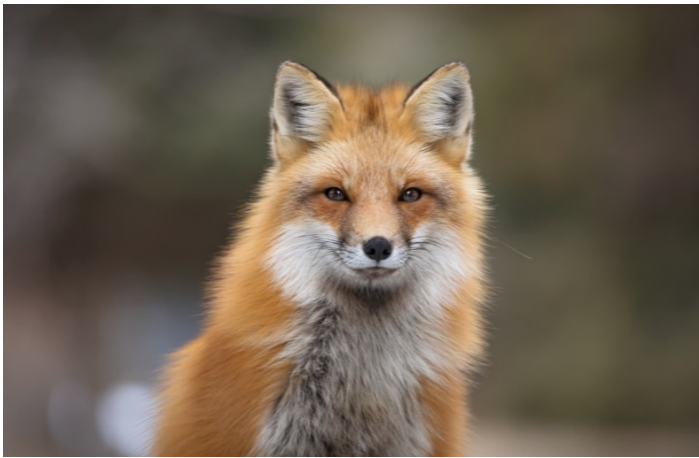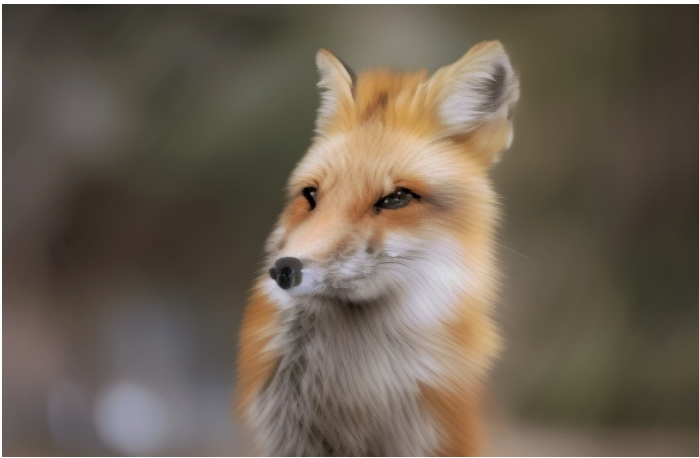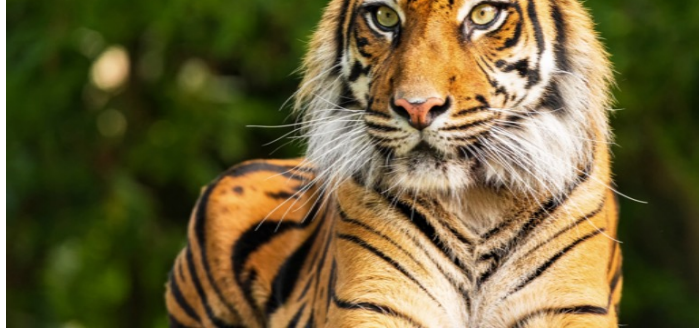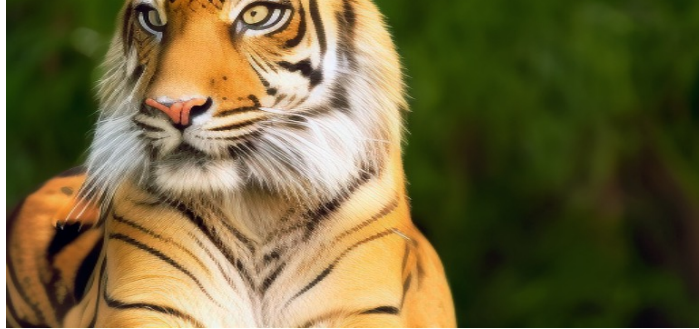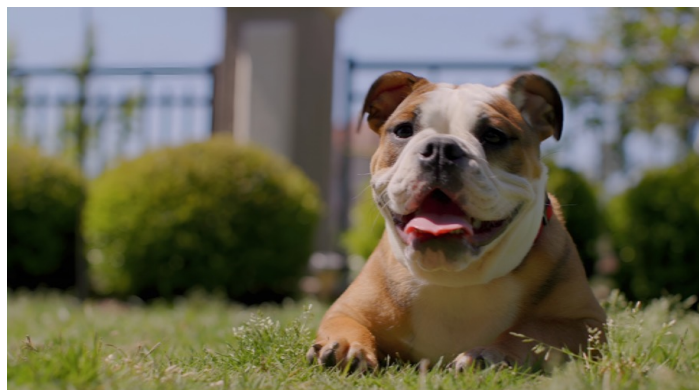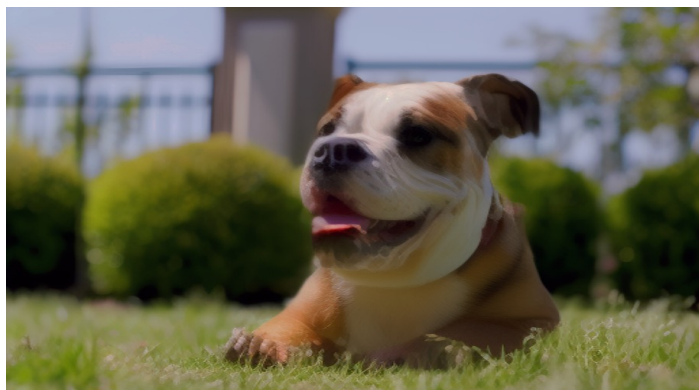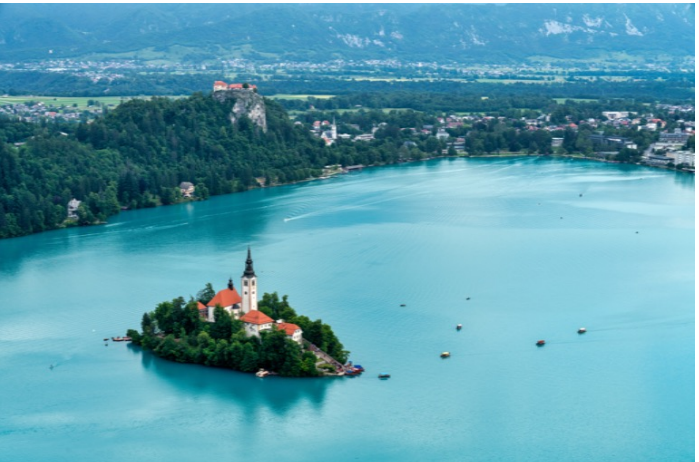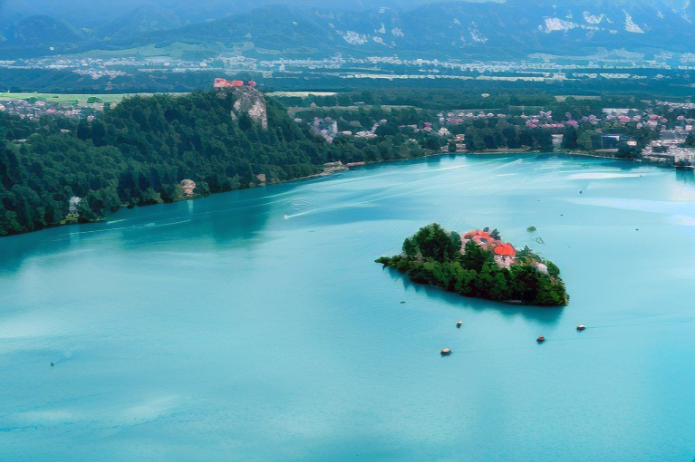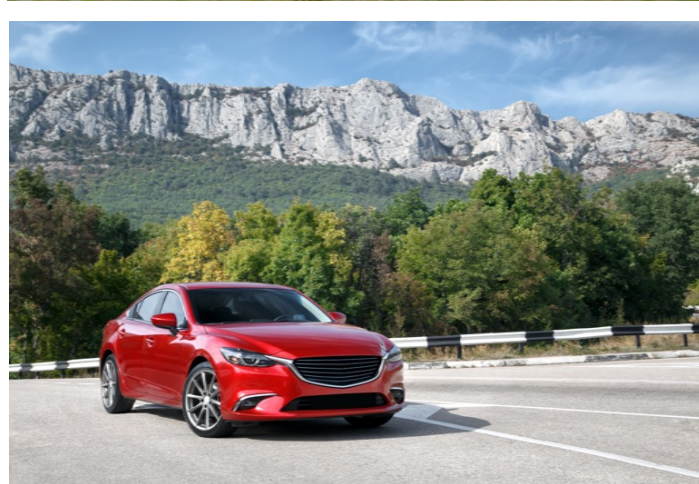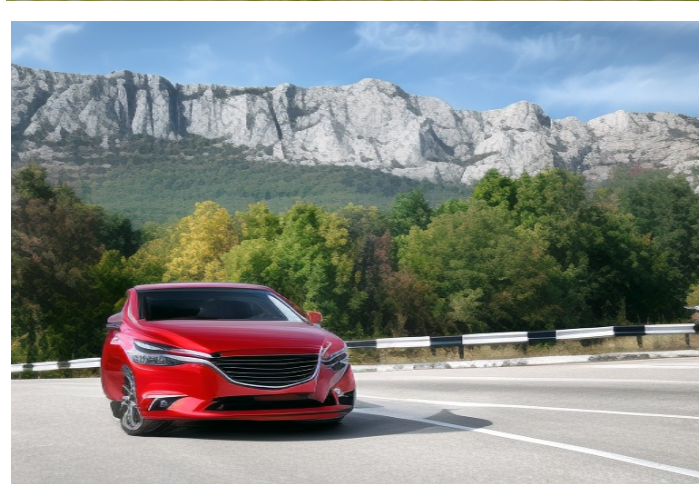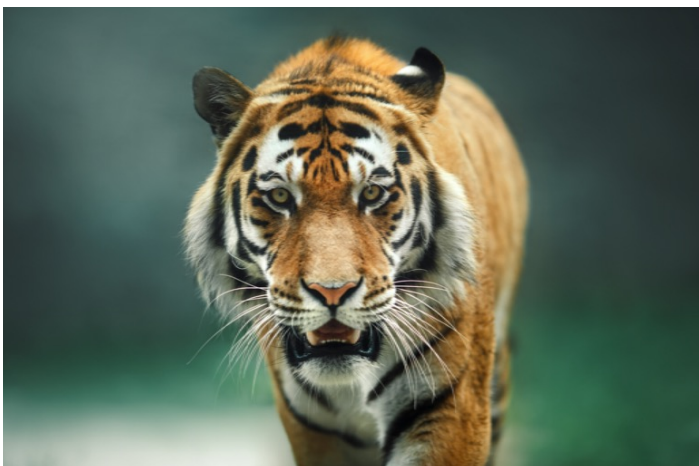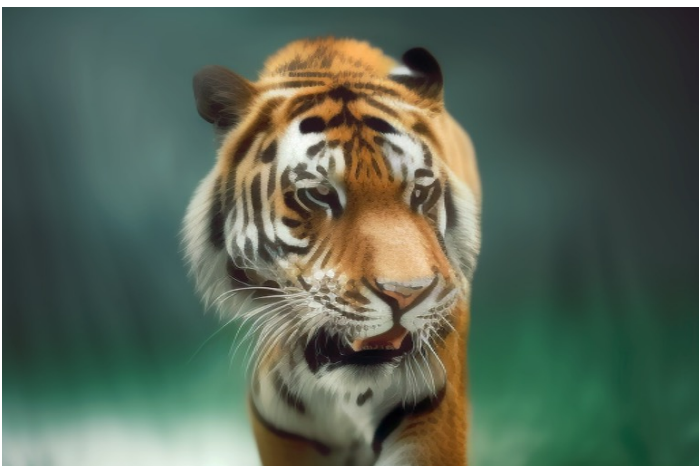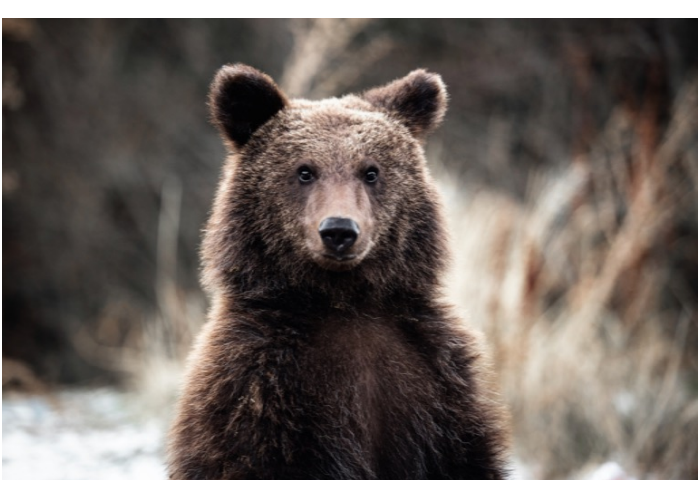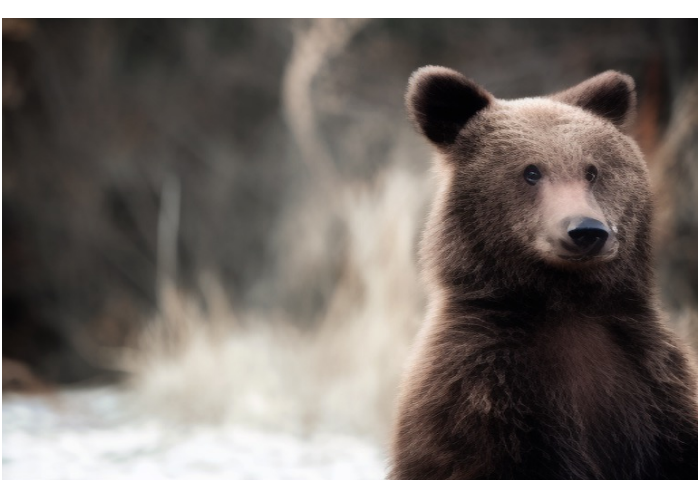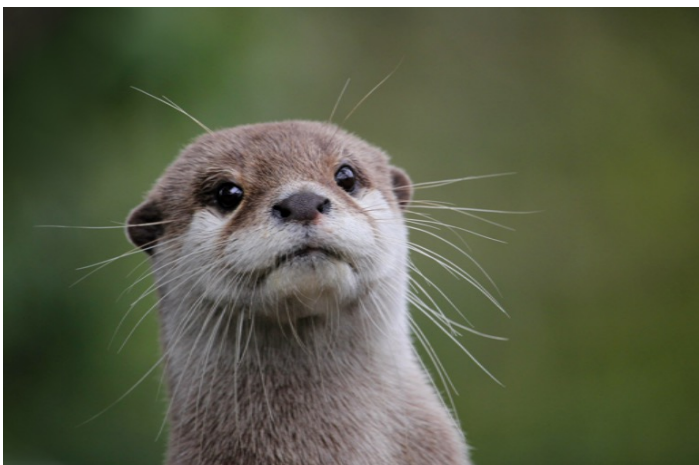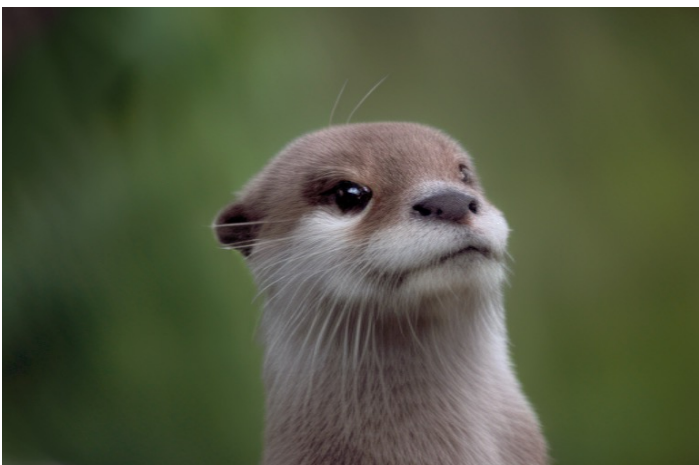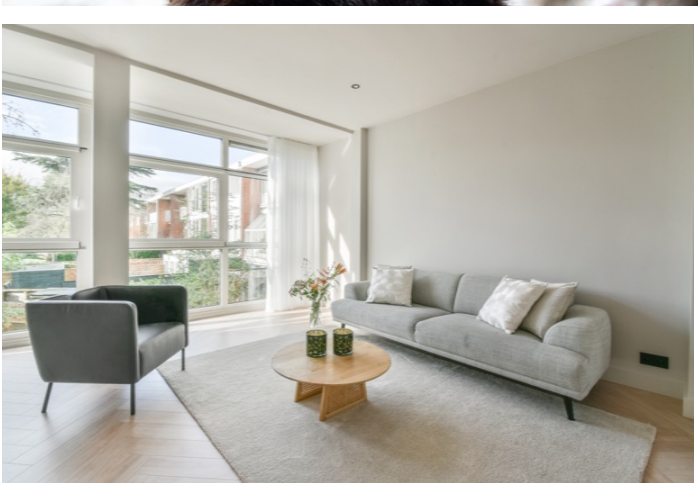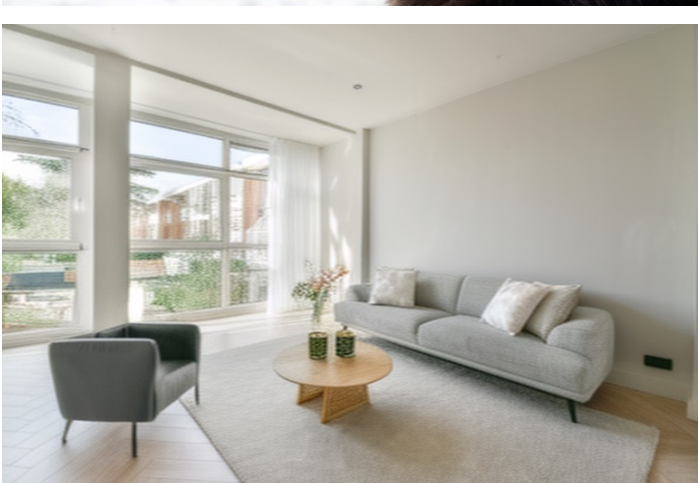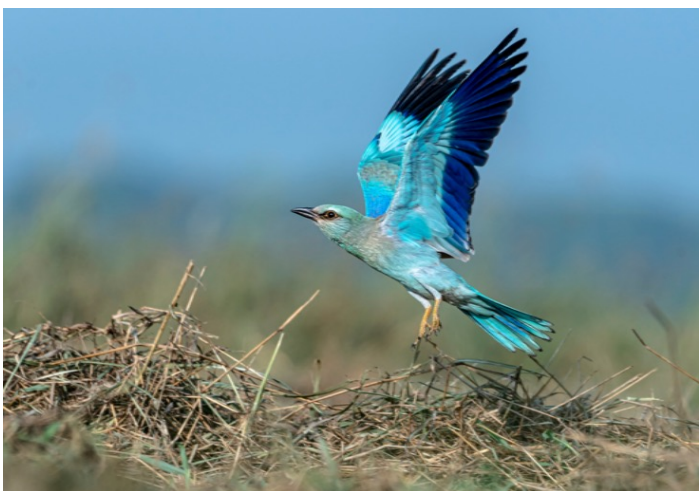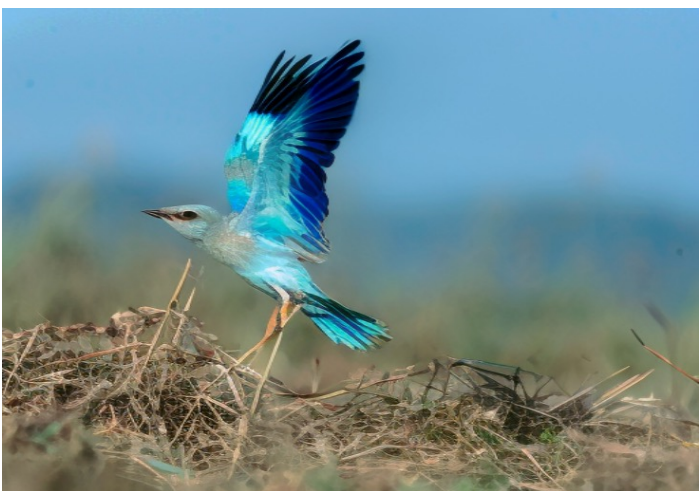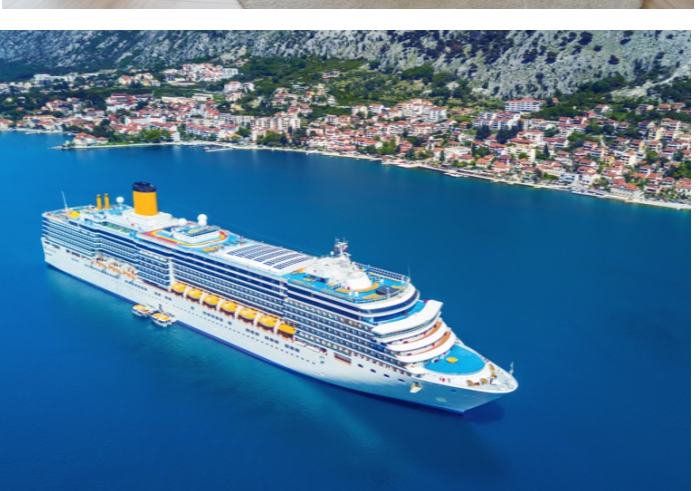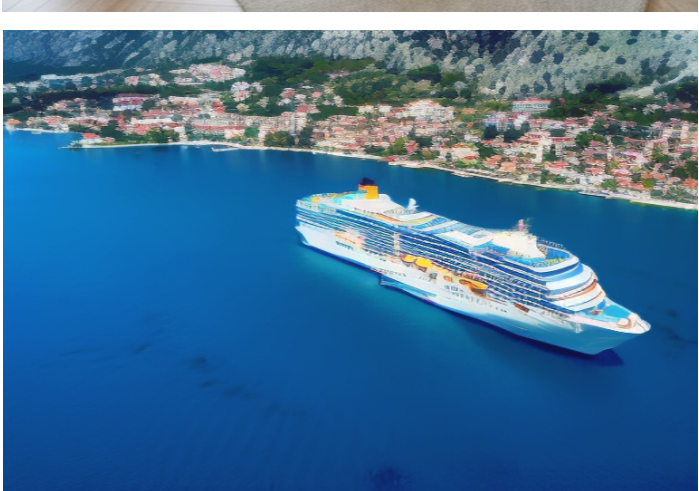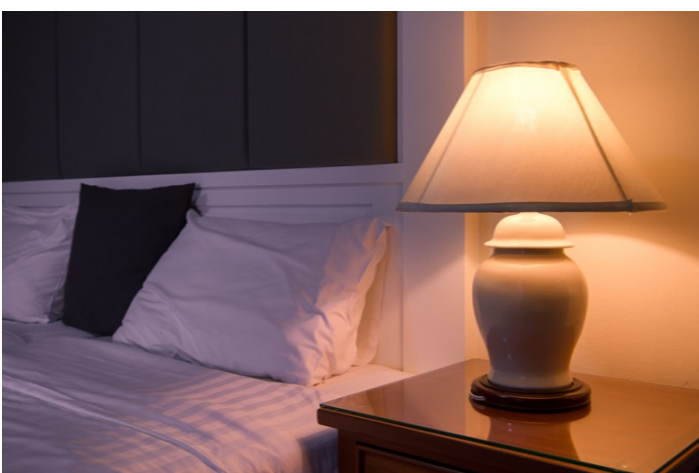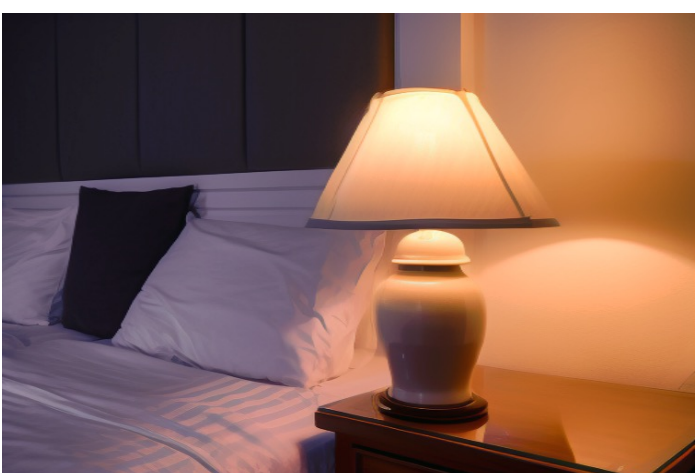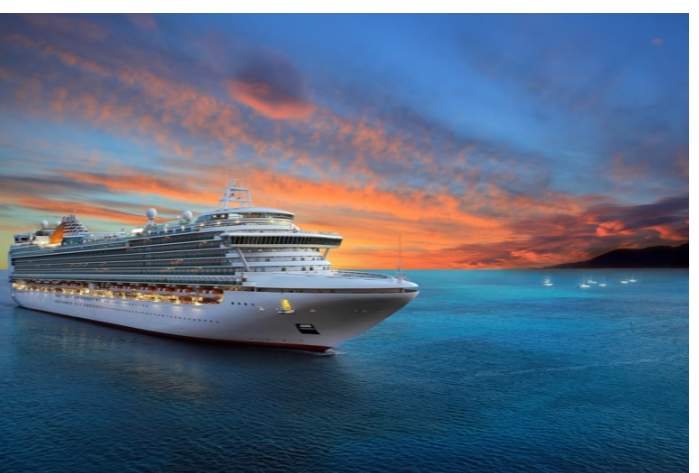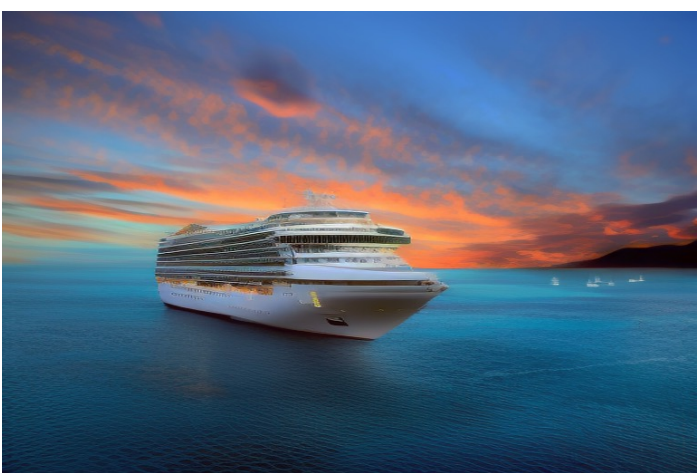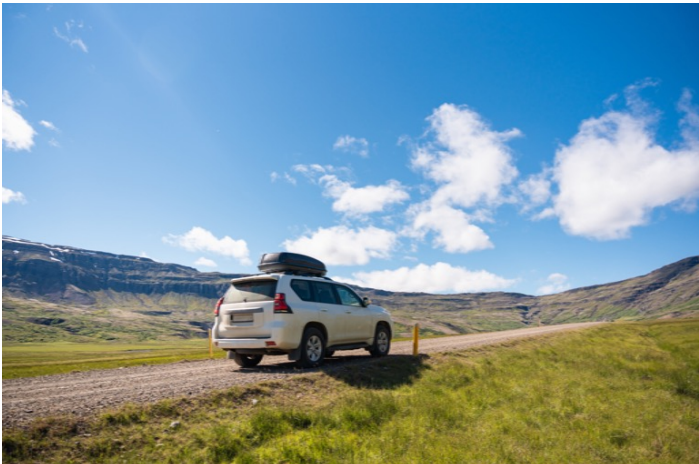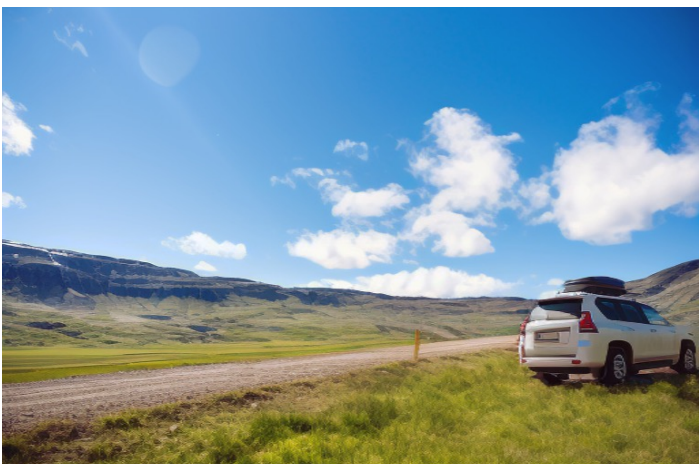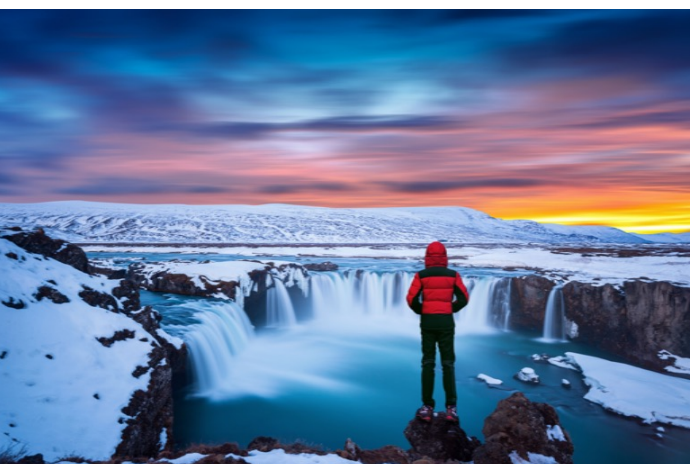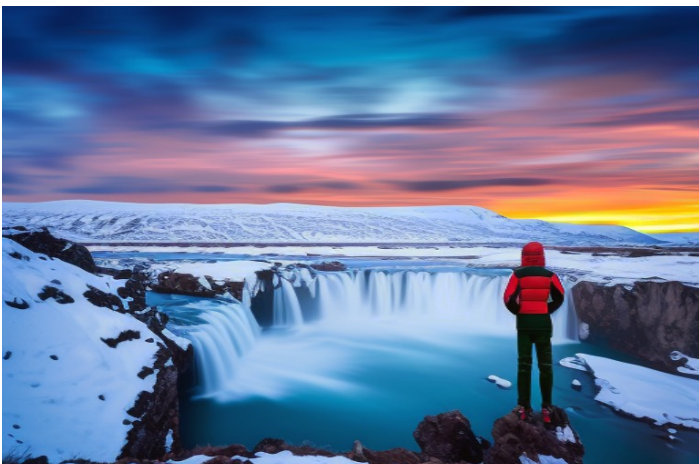



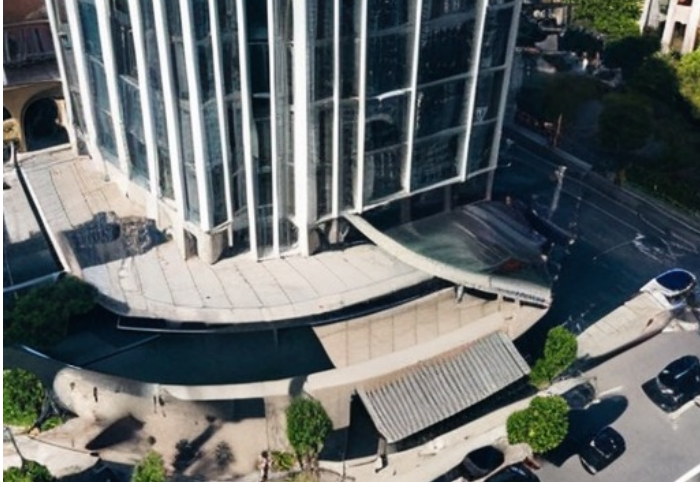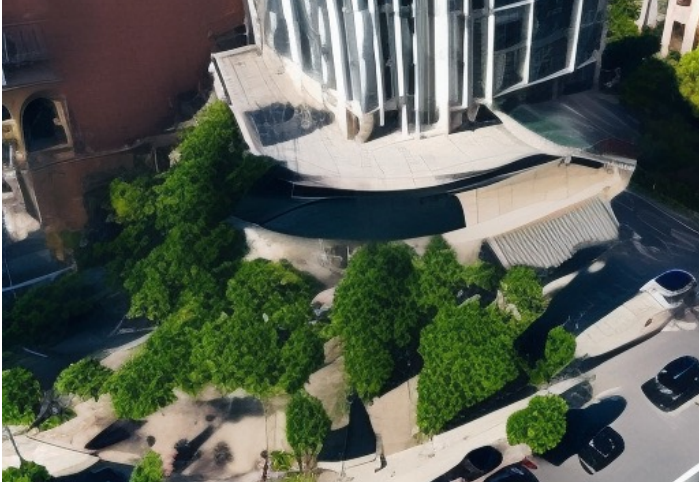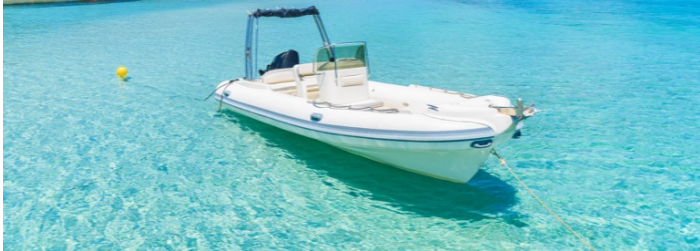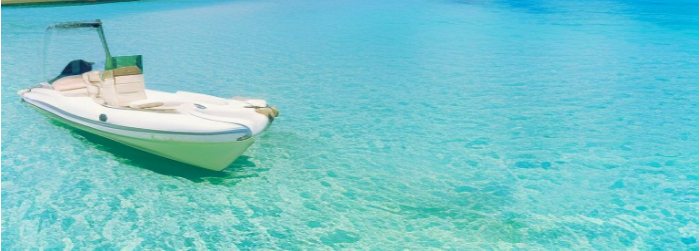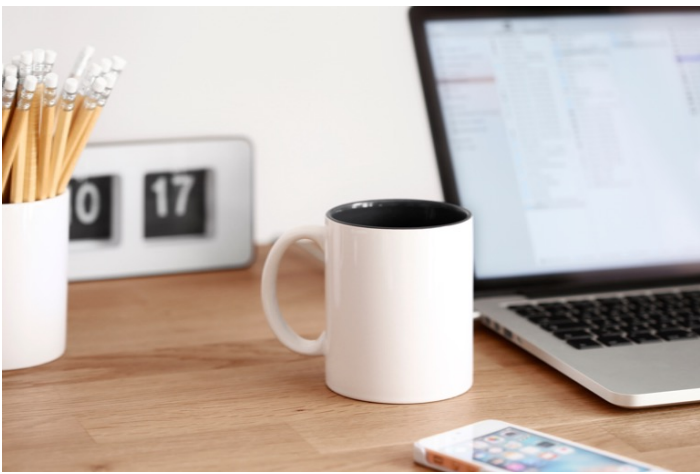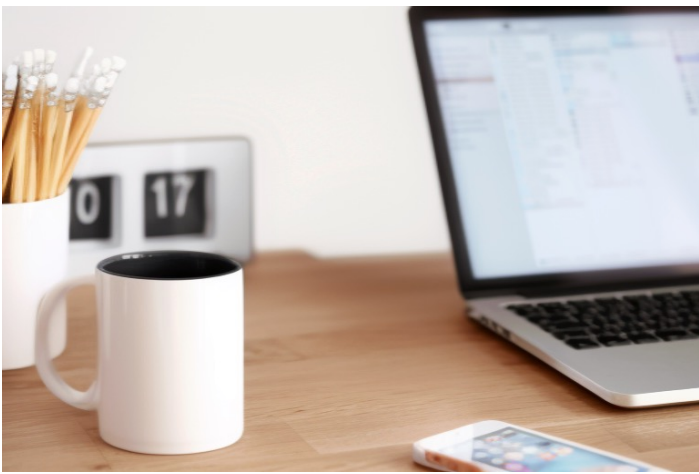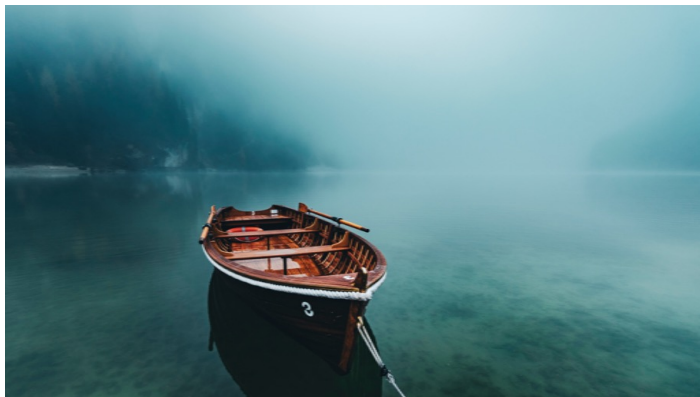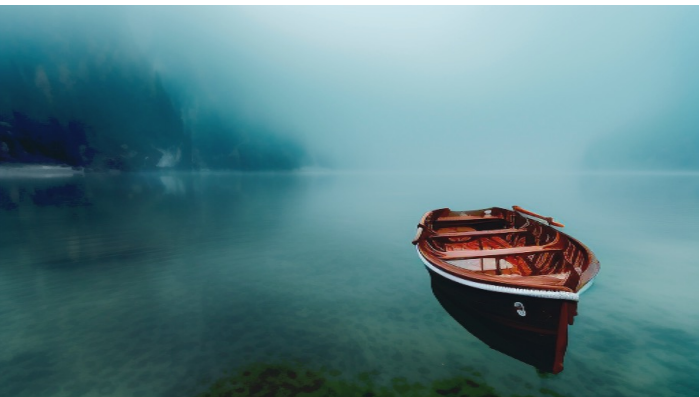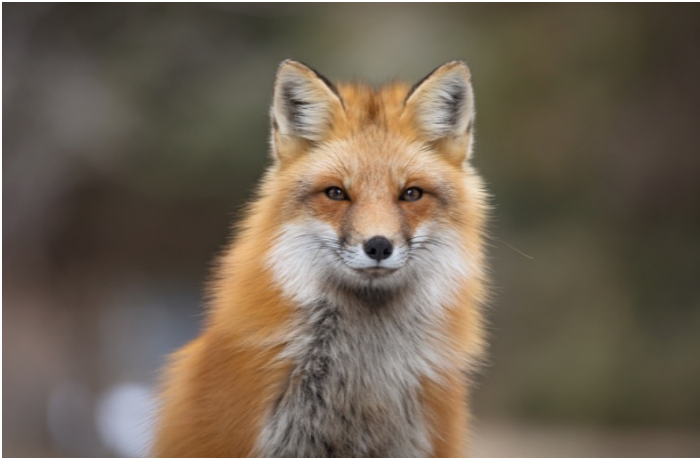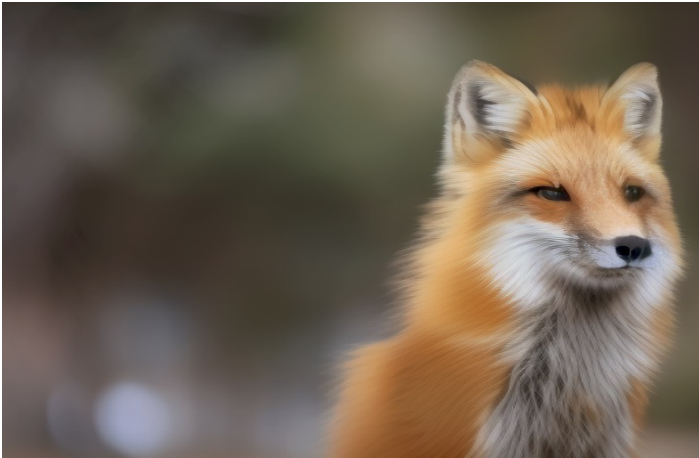

Supplement: Supplementary file 1 [file Gallery_supp_2.pdf]
